# Supplementary material for: FOCAL: A Cost-Aware Video Dataset for Active Learning
Source: arXiv:2311.10591 source file (2023-11-17)
Supplement: Supplementary file 1 [file AppendixA.tex]

\subsection{Links to Access Dataset} \label{app:link}
The hosting of the dataset will exist within the IEEE Dataport platform. Release of the full dataset and associated code will occur shortly after notification of acceptance.

\subsection{Dataset Folder Structure} \label{app:structure}
The structure of the dataset folder is illustrated in the Figure~\ref{fig: folder_structure}. There are two major folders under the root directory, including images and labels. The training, validation and test sub-folders under the labels directory contains the frame-wise annotation files associated with the image files under the corresponding sub-folders under the images folder.

\begin{figure}[h!]
\centering
\includegraphics[scale=0.5]{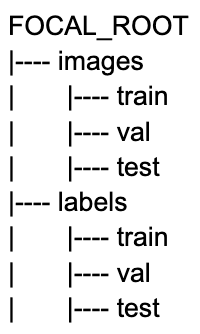}

\caption{The structure of the data folder.\vspace{-.3cm}}

\label{fig: folder_structure}
\end{figure}

\subsection{Naming Conventions} \label{app:names}
The label files are named with the same naming conventions as those of the image files. Specifically, the naming convention of the annotation files is: $<sequence ID>\_<frame ID>.txt$. Similarly, the naming convention of the image files is: $<sequence ID>\_<frame ID>.jpg$. 

\subsection{Box Annotation Format} \label{app:format}
Each individual annotation text file contains the  bounding box coordinates of all objects within the associated frame as mentioned in the above naming conventions. Specifically, the bounding box annotations take the format as $<object\ class>\ <x_{center}>\ <y_{center}>\ <width>\ <height>$.
