# Supplementary material for: FOCAL: A Cost-Aware Video Dataset for Active Learning
Source: arXiv:2311.10591 source file (2023-11-17)
Supplement: Supplementary file 2 [file AppendixC.tex]

We elaborate on the details of the key aspects of the dataset in this section. 
\subsection{Object labels}
%% \paragraph{Object Labels}
The data in \texttt{FOCAL} was captured from stationary cameras at different places. All data taken from the mounted cameras were fed into a labeling platform. Image data was fed into a tool to anonymize sensitive information, e.g., blurring the faces of pedestrians and the license plates of vehicles. Every sequence was then labeled by annotators for 2D bounding box coordinates, tracking identities, and state annotations for various agent interactions, such as whether a vehicle is parked or not. These annotations took place at a rate of 10 Hz. Objects were labeled to be one of 23 possible classes as shown by the left graph in Figure \ref{fig: class_cost_dist}.  In our active learning experiments, the 23 classes have been consolidated into 4 superclasses including Pedestrian, Bicycle, Car, and Cart. 
% After annotations were completed for an individual sequence, the sequence was sent for review to a separate team who performed quality assurance for the curated annotations. 
% The separation between quality assurance and the first-stage annotation  minimizes bias in annotations. 

During the annotation process for each sequence, time information regarding the usage of the labeling platform by each annotator is tracked. The annotation cost label of a sequence is the cumulative time of all users that performed any labeling or quality assurance on the sequence. The cost for each sequence varies as shown by the right graph in Figure~\ref{fig: class_cost_dist}, where we show a histogram of the time spent labeling in hours compared to the number of sequences in the dataset. The variation in the annotation-cost time   indicates that the \texttt{FOCAL} dataset contains both hard and easy sequences to label. This is beneficial for distinguishing active learning strategies, i.e., an optimal strategy should select the sequences with less time to annotate over others, while simultaneously optimizing for performance.

\begin{figure*}[t]
\centering
\includegraphics[scale = .65]{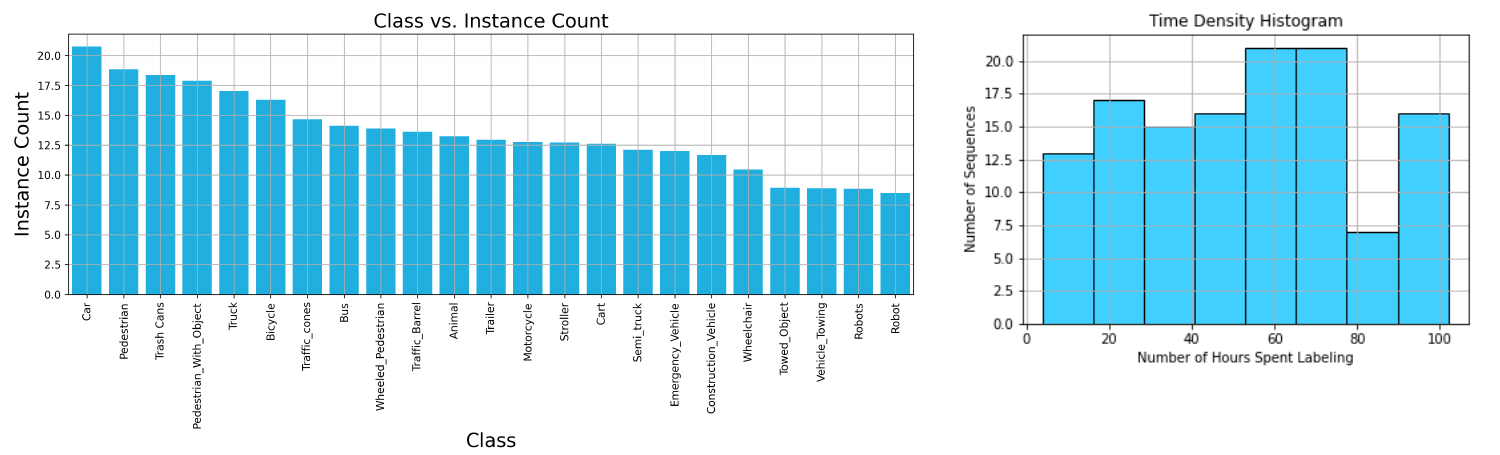}

\caption{\texttt{FOCAL} dataset class distribution and variation of cost annotations. Left: Log-scaled class distribution. The y-axis shows the number of object instances for each class in the \texttt{FOCAL} dataset. Right: Variation of cost within frames in sequence. The variation is beneficial for distinguishing active learning algorithms to identify optimal strategies that simultaneously select sequences with less time to annotate and optimize for performance.\vspace{-.3cm}}

\label{fig: class_cost_dist}
\end{figure*}

\subsection{Meta Data}
% \paragraph{Metadata} 
There is a variety of associated metadata specific to the type of object in the label file for each sequence. For vehicles, the associated metadata includes a state label that is indicative of parking or not. For pedestrians, there are labels indicating whether the person is walking or standing. Finally, there is an occlusion label for every object. The occlusion label indicates whether the associated object is hidden behind another object, partially hidden, or fully visible within the current frame.

\subsection{Scene Diversity}
% \paragraph{Scene Diversity} 
In order to obtain training, test, and validation sequences in non-overlapping scenes, we manually group all sequences into 69 unique scenes according to their geographic locations. We assign each scene a unique identifier. The sequences collected at the same scene are associated with the same scene identifier. The statistics of scene identities are shown in Figure \ref{fig: scene_id}. In addition to location diversity, sequences in \texttt{FOCAL} also contain varied environmental conditions. The sequences were collected in a wide range of seasons from winter to summer. The ratio of each season is depicted in Figure \ref{fig: season_pie}. Overall, there are 10.30\%, 63.49\%, and 26.21\% sequences collected in the winter, spring, and summer, respectively. In summary, our scene selection encourages diverse data conditions to evaluate active learning algorithms.

\begin{figure}[h!]
\centering
\includegraphics[width = 6in]{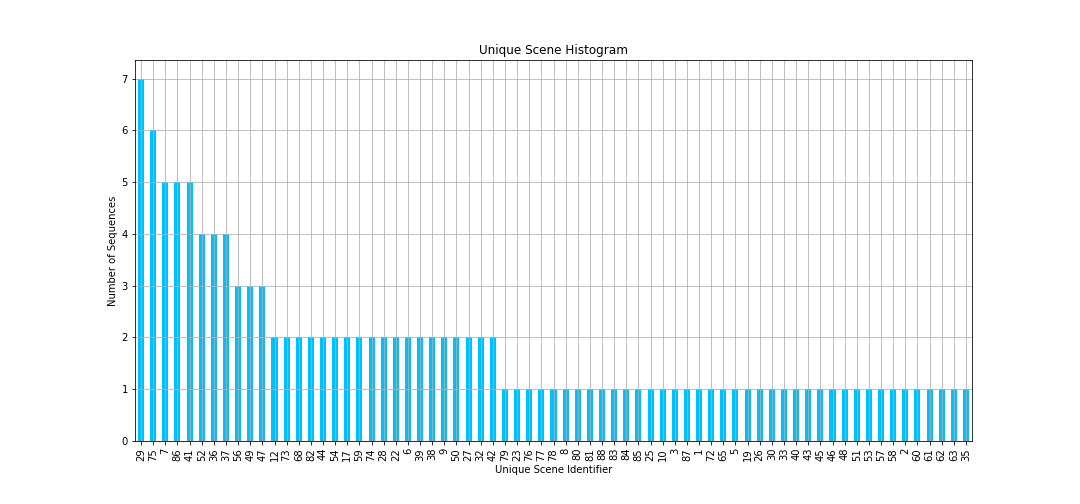}

\caption{Unique scene identities. All sequences are grouped into 69 unique scenes to obtain non-overlapping training and test scenes. The x-axis represents assigned scene identities. The y-axis shows the number of sequences collected at each corresponding scene.\vspace{-.3cm}}

\label{fig: scene_id}
\end{figure}

\begin{figure}[h!]
\centering
\includegraphics[scale=.35]{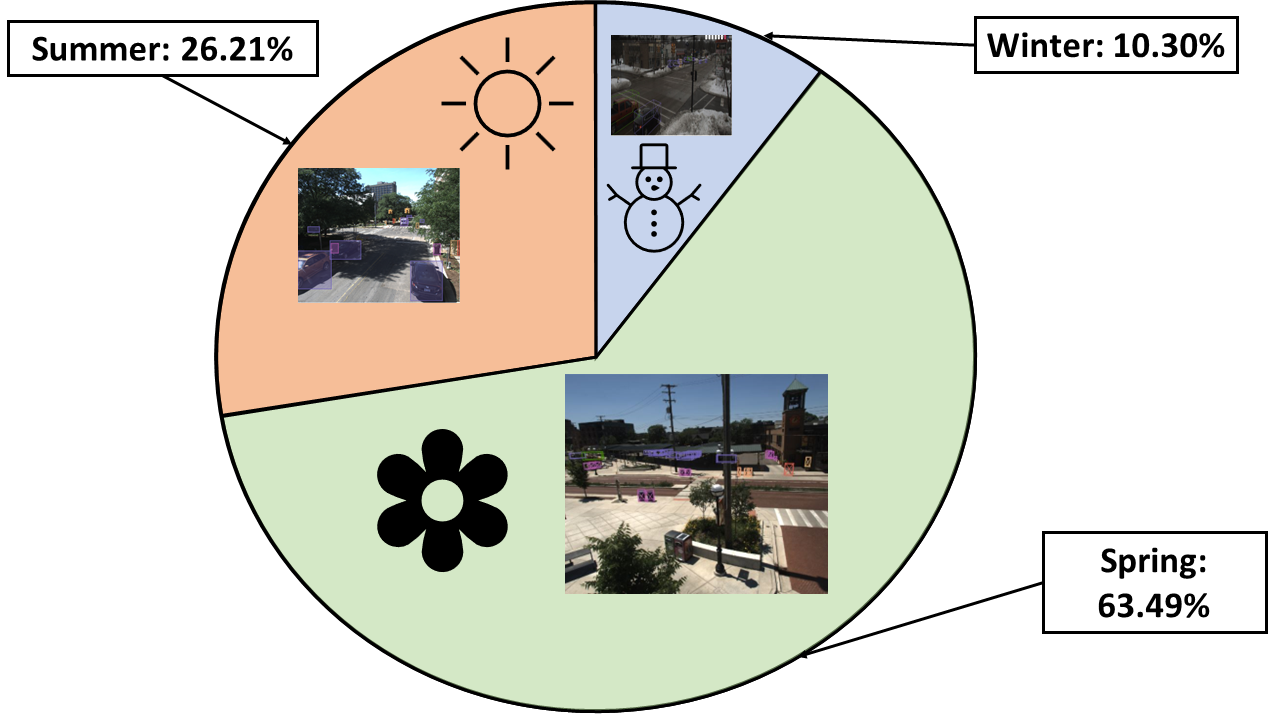}

\caption{Season distribution in the \texttt{FOCAL} dataset. The sequences were collected in multiple seasons to encourage diverse environmental conditions and object activities.\vspace{-.3cm}}

\label{fig: season_pie}
\end{figure}

\subsection{Object Diversity}
% \paragraph{Object Diversity} 
In addition to the scene diversity, object diversity is also present in the \texttt{FOCAL} dataset. As shown in the left graph in Figure \ref{fig: class_cost_dist}, the overall semantic categories include various types of pedestrians, vehicles, static scene objects, etc. Furthermore, Figure \ref{fig: obj_density} illustrates the statistics of averaged object quantity per frame across all sequences. Due to the variation in locations and environmental conditions, the number of object instances varies across different sequences. For instance, the sequences collected in the summer contain more objects with diverse activities compared to the sequences collected in the winter. This object density variation is beneficial to the evaluation of active learning algorithms. 

\begin{figure}[h!]
\centering
\includegraphics[scale = .8]{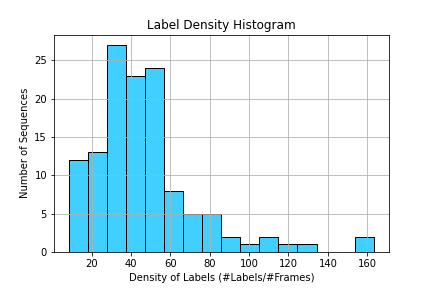}

\caption{Object instance density. Object diversity is presented in the \texttt{FOCAL} dataset.\vspace{-.3cm}}

\label{fig: obj_density}
\end{figure}

\subsection{Frame Quantity Distribution}

\subsubsection{Frame Quantity Distribution}
We show the distribution of frame quantity for all sequences in Figure \ref{fig: frame_dist}. The majority of sequences are constrained within 594 to 864 frames, indicating that the sequences contain a relatively equal number of frames. This avoids bias in terms of utilizing sequence length as a major indicator for active learning. Ideally, active learning algorithms should utilize the inherent information and difficulties with labeling to achieve high generalization and low annotation cost, instead of querying according to the variation of sequence length.

\begin{figure}[h!]
\centering
\includegraphics[scale = .75]{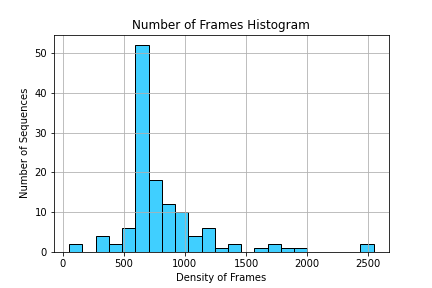}

\caption{Variation of frame quantity in sequences. The majority of collected sequences consist of a relatively equal number of frames. This avoids potential bias in terms of sequence length in querying strategies.\vspace{-.3cm}}

\label{fig: frame_dist}
\end{figure}

\subsection{Change of Object Quantity}
\subsubsection{Change of Object Quantity}
The temporal first-order statistics of the accumulative object quantity can be considered as a factor of annotation cost. Specifically, we calculate such statistics as the change of object quantity between a certain fixed number of frames, as shown in Fig~\ref{fig: change_objquant}. A higher number of mobile objects moving in and out of the field of view can result in higher annotation costs due to more efforts in accurately tracking these objects.

\begin{figure}[h!]
\centering
\includegraphics[scale=0.7]{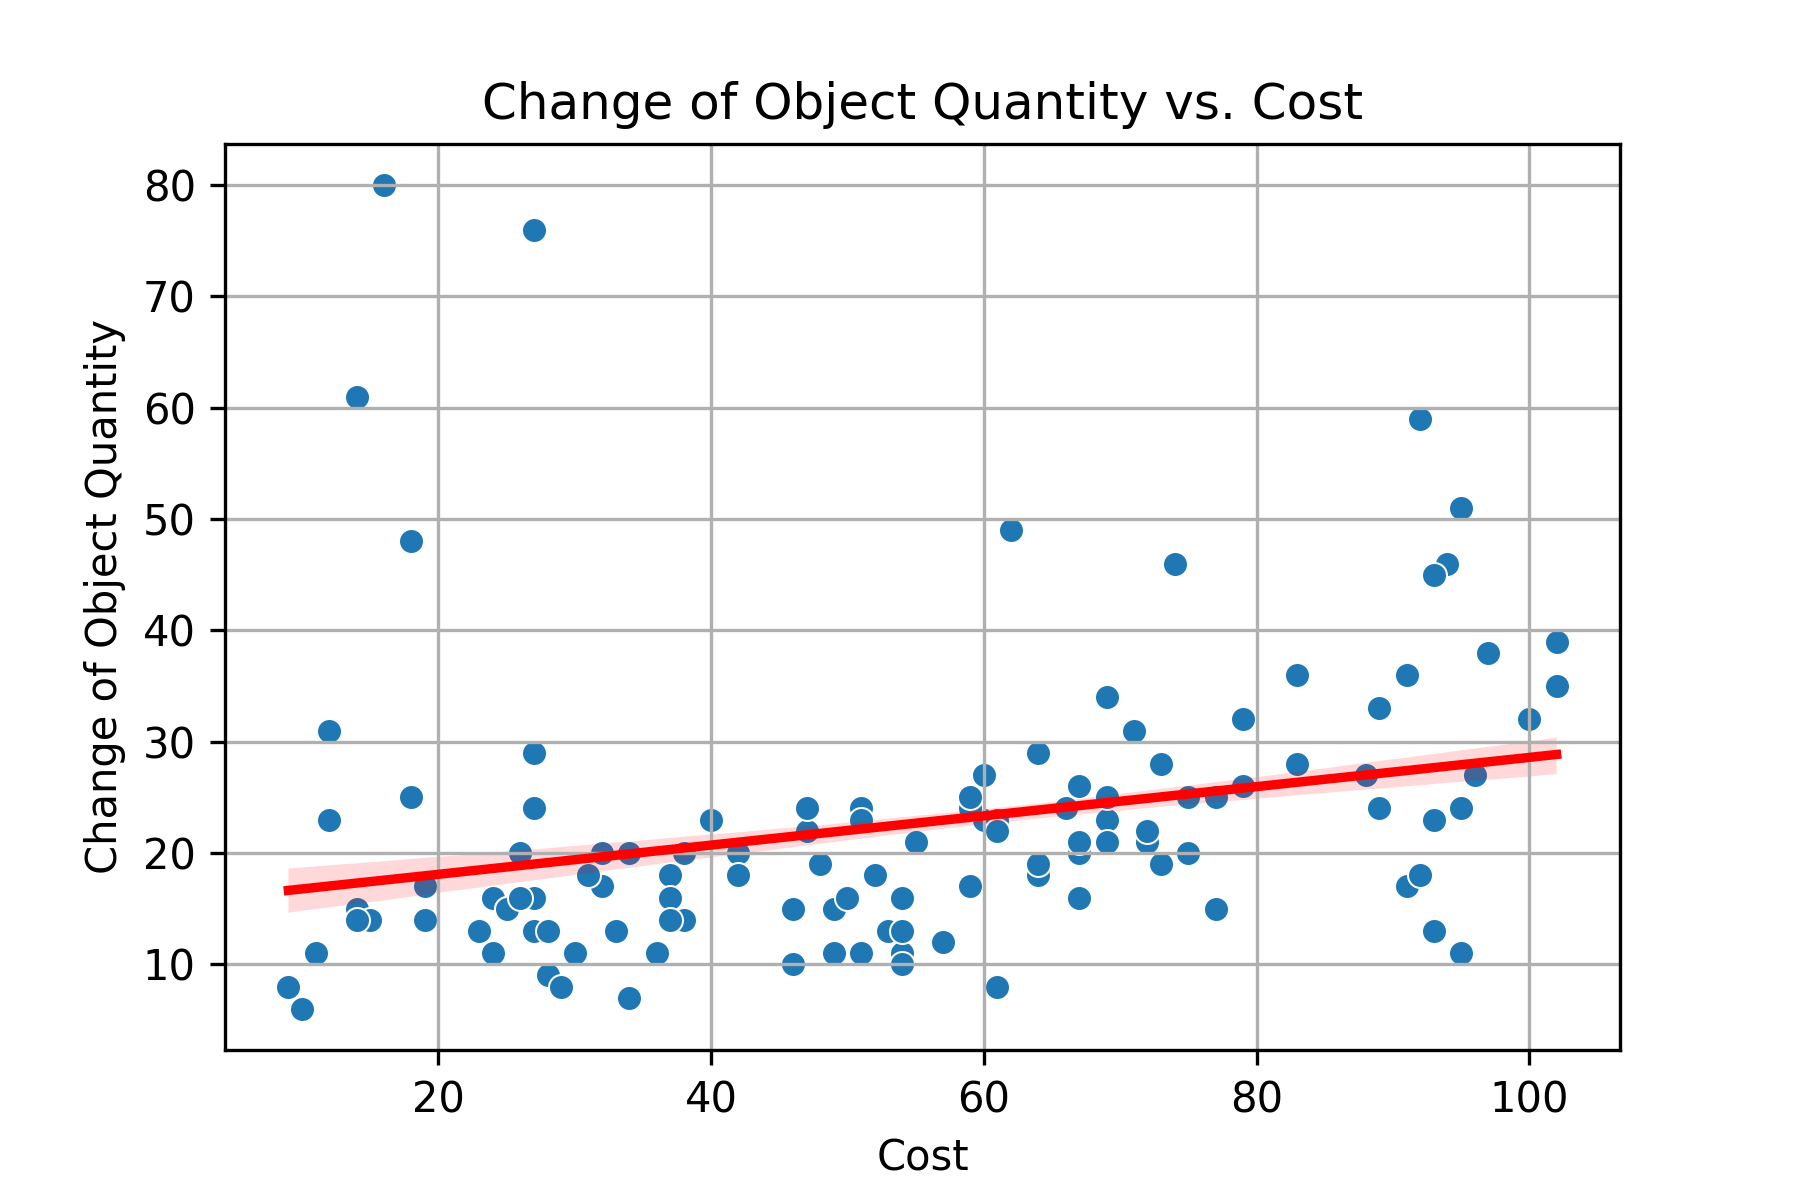}

\caption{Change of object quantity.\vspace{-.3cm}}

\label{fig: change_objquant}
\end{figure}

\subsection{Estimated Statistics} 
Figure \ref{fig:est_queries}(a,b) shows the relationship between estimated motion and estimated box count \texttt{FOCAL} statistics with cost. Conformal sampling algorithms are based on these relationships with cost.

\begin{figure} [h!]
\centering
\includegraphics[width=\textwidth]{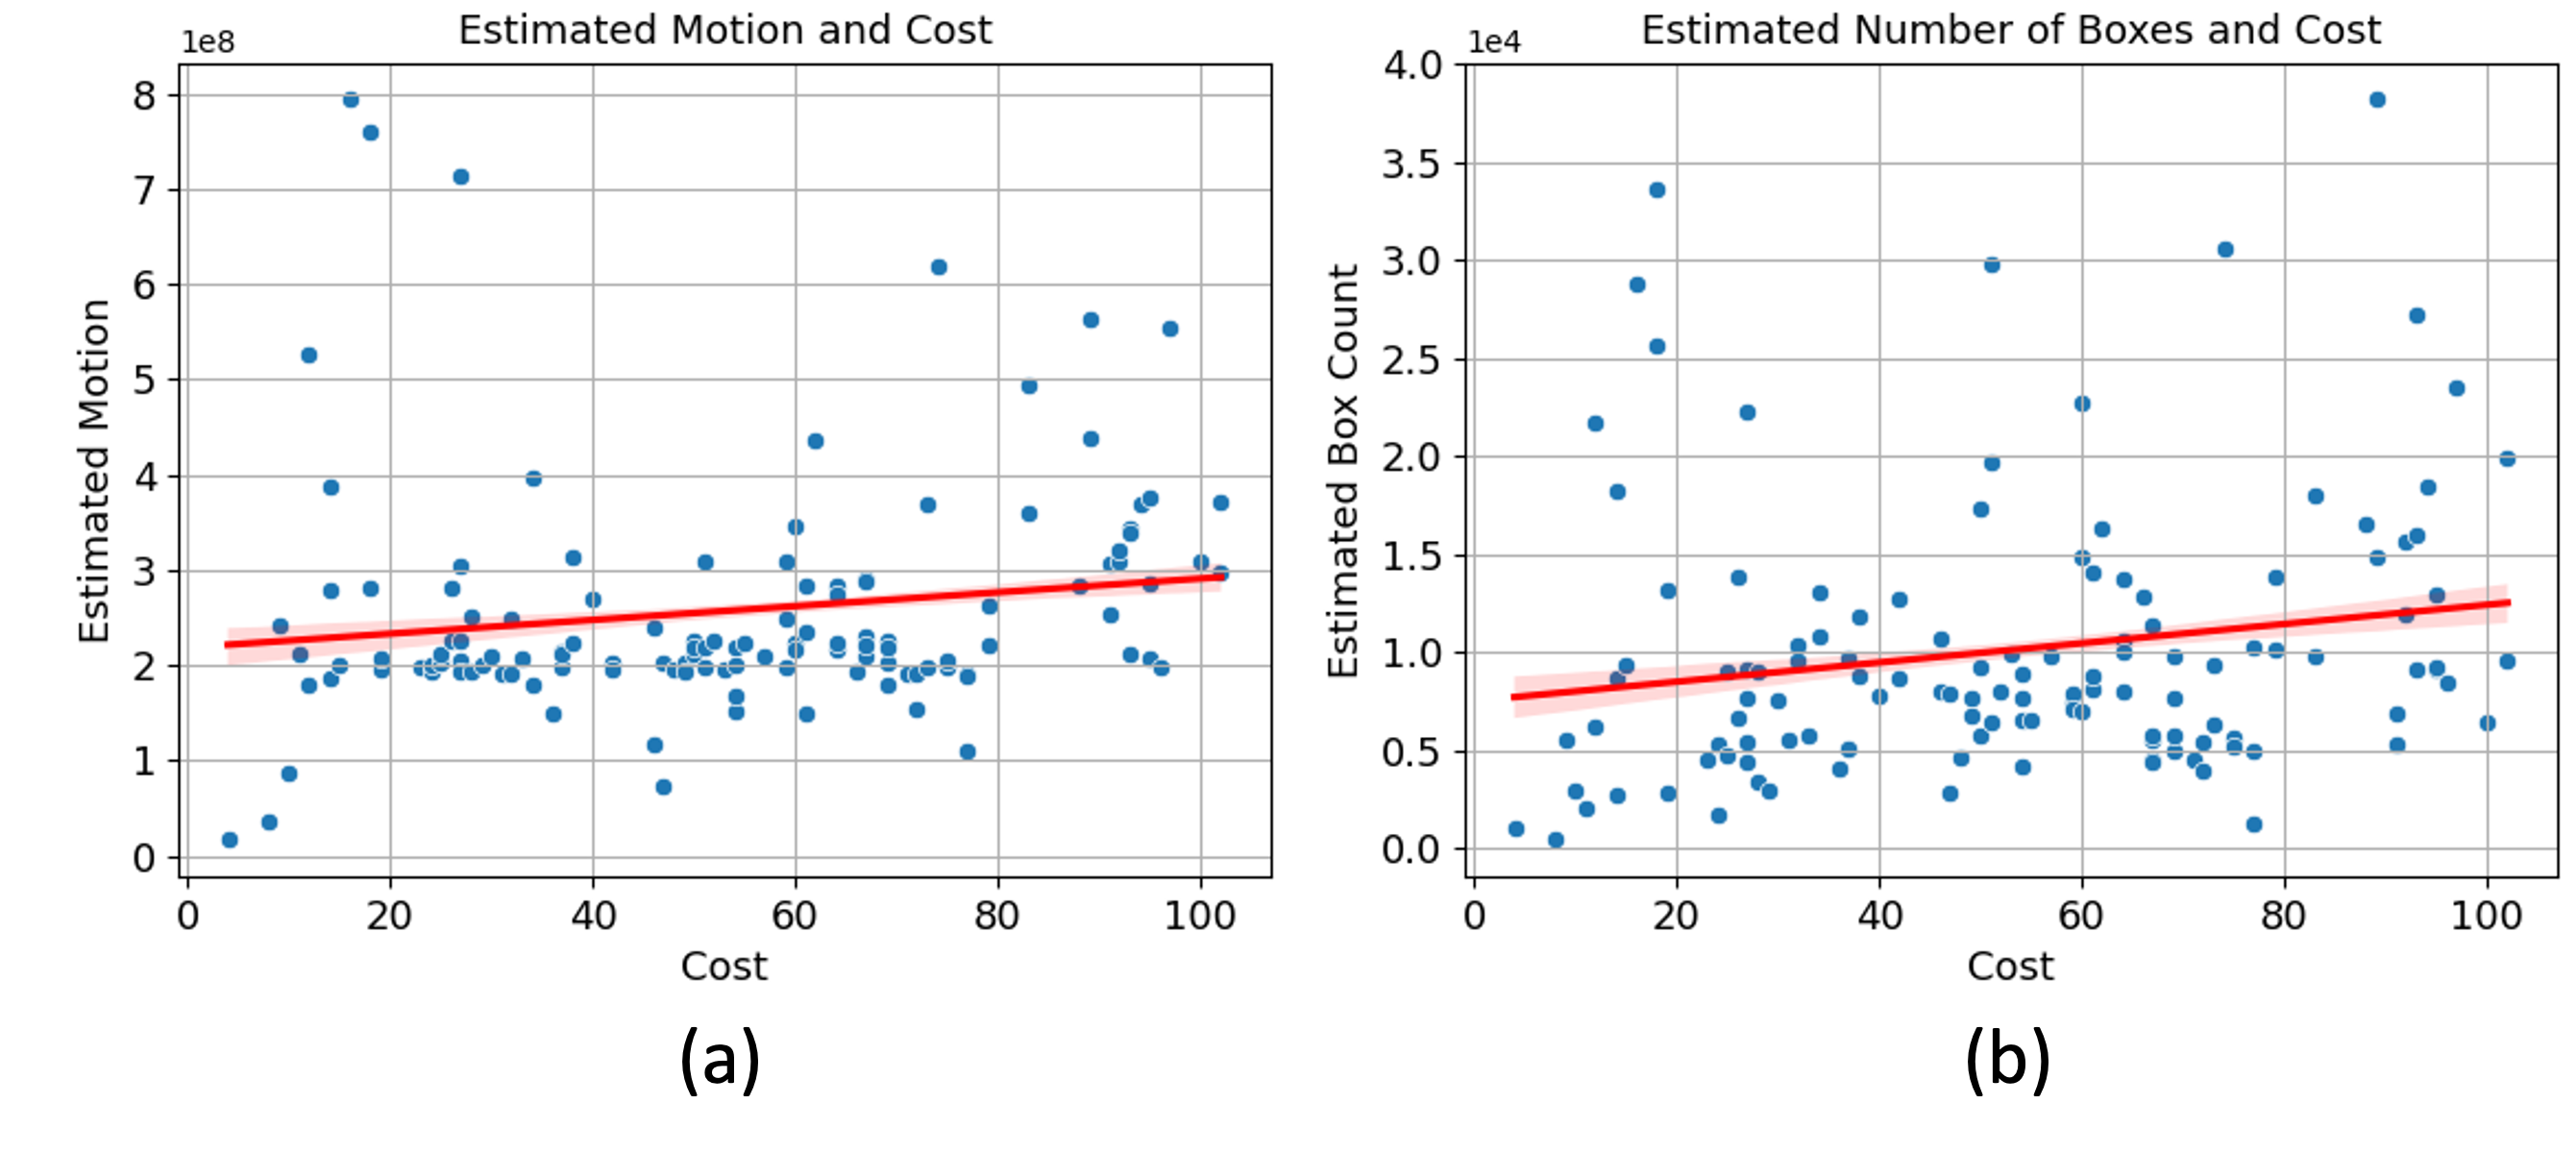}
\caption{(a) The relationship between estimated motion (derived from optical flow) and cost. (b) The relationship between estimated box count (also derived from optical flow) and cost.}
\label{fig:est_queries}
\end{figure}
