# Supplementary material for: FOCAL: A Cost-Aware Video Dataset for Active Learning
Source: arXiv:2311.10591 source file (2023-11-17)
Supplement: Supplementary file 3 [file AppendixD.tex]

We provide additional details about the experimental setup of object detection and sequence active learning in this section.

\subsection{ Object Detection and Sequence Active Learning}
The same data splits are used for both object detection and sequence active learning. All images are resized to a $640\times640$ pixel resolution during training, validation, and inference. Objects that have associated bounding boxes with both height and width smaller than $50$ pixels are not used for training, testing or validation. All architectures are initialized with the weights of the models pretrained on the COCO Dataset \cite{lin2014microsoft}. Model optimization is performed using stochastic gradient descent with an initial learning rate of 0.01 and follows a cosine learning rate scheduler as training progresses. During inference, we use the optimal weights with respect to the validation set to evaluate the model's performance on the test data. 

% \subsection{Performance-Cost Metrics}

% \paragraph{Cost Appreciation Rate}
% The cost appreciation rate is the area under the mAP vs cost curve at different cost budgets. CAR is defined as follows:

% \begin{equation}
% \label{eq:car}
%     CAR = \int_{0}^{b} AP({c}) \,dc.
% \end{equation}

% where $b$ is the cost budget, $c$ is a cost value less than the budget, and AP({c}) is the corresponding mAP on the y-axis for cost value $c$.

% \paragraph{Performance Appreciation Rate}
% Similar to CAR, the performance appreciations rate is the area under the mAP vs cost curve at different performance budgets. PAR is defined as follows:

% \begin{equation}
% \label{eq:car}
%     PAR = \int_{0}^{b} AP({p}) \,dp.
% \end{equation}

% where $b$ is now the performance budget, $p$ is a performance value less than the budget, and $AP({p})$ is the corresponding cost on the x-axis for performance value $p$. 
