# Supplementary material for: FOCAL: A Cost-Aware Video Dataset for Active Learning
Source: arXiv:2311.10591 source file (2023-11-17)
Supplement: Supplementary file 4 [file appendix.tex]

\section{Supplementary Material}
\subsection{Dataset Access}
% The dataset and associated code can be found at https://github.com/olivesgatech/FOCAL.

The hosting of the dataset will exist within the IEEE Dataport platform. Release of the full dataset and associated code will occur shortly after notification of acceptance.
\subsection{Dataset Labeling Details}
Within this section, we show specific details surrounding the labeling process. After the data is entered into the online annotation platform, the annotator uses the setup shown in Figure \ref{fig: real_labeling} in order to assign bounding boxes to the objects in the scene as well as interpolate these objects across the sequence.
Also within this annotation tool is a system to track the amount of time each user spends working on a sequence. This is shown through the example for a specific sequence in Figure \ref{fig: real_labeling_time}. The x-axis shows the dates in which work on the sequence was performed and the y-axis indicates the number of cumulative hours across all users for that specific sequence. This work is divided into quality assurance and annotation time and the sum across all hours worked on each date is the final labeling time for the sequence. This can be further understood through the data files available in the dataset. Figure \ref{fig: sequence_screenshot} shows how every sequence comes with its own identity as well as information regarding frames, quantity of bounding boxes, unique scene identifier, and the cumulative number of days and hours it took to label the sequence. Participants who annotated the data and performed quality assurance were compensated appropriately for their services.

\subsection{Dataset Cost Acquisition}

In Figure \ref{fig: cost_comp}, we provide an overview of how we obtained the cost label for every sequence. 
\begin{figure}[h!]
\centering
\includegraphics[width = \columnwidth]{Fig/Van Images/labeling.png}

\caption{Example of labeling setup within our internal platform.\vspace{-.3cm}}

\label{fig: real_labeling}
\end{figure}

\begin{figure}[h!]
\centering
\includegraphics[width = \columnwidth]{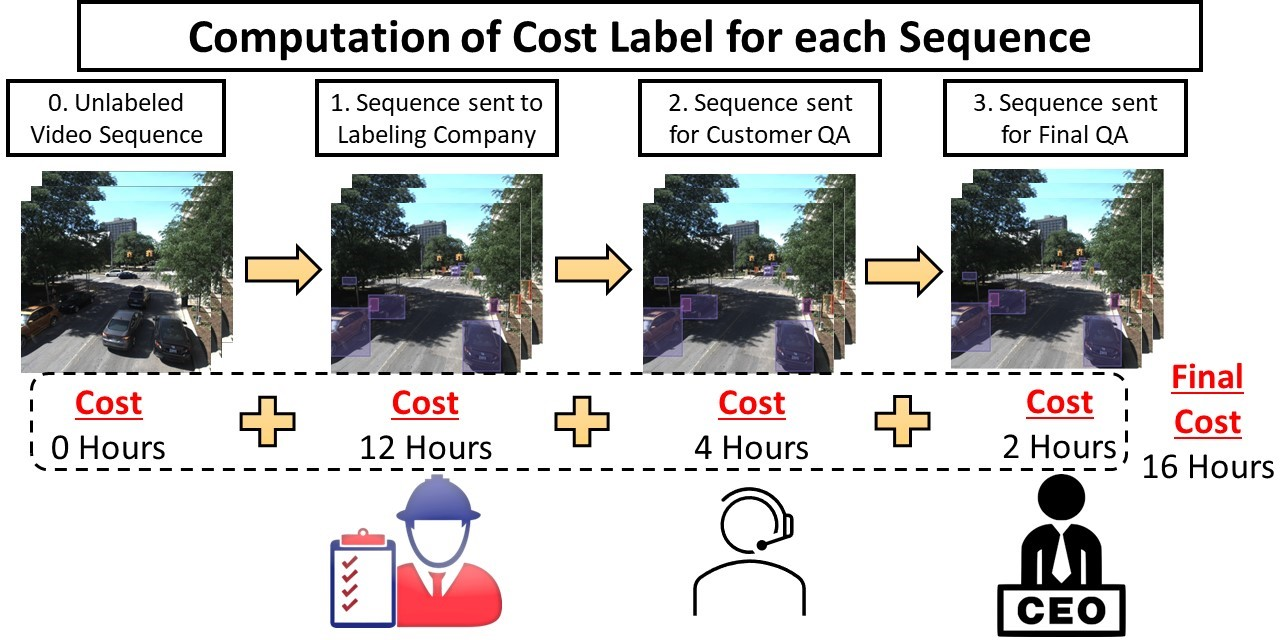}

\caption{Process by which cost is computed is computed.\vspace{-.3cm}}

\label{fig: cost_comp}
\end{figure}

\begin{figure}[h!]
\centering
\includegraphics[width = \columnwidth]{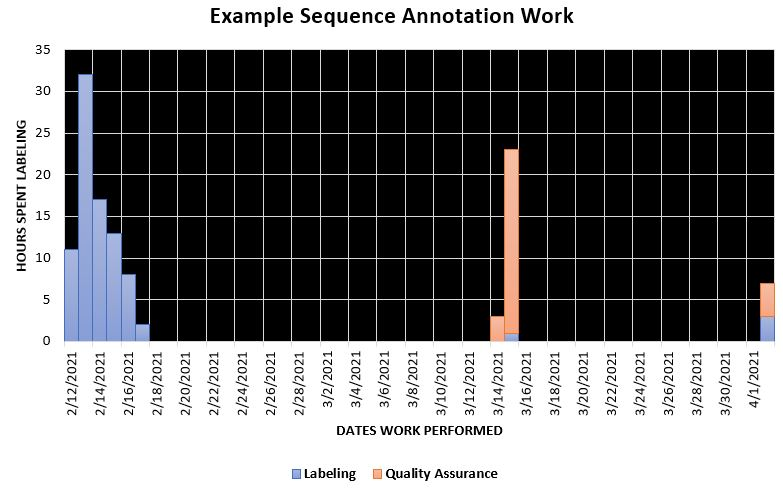}

\caption{Example of how cost annotation is calculated within the labeling tool. Users log in on specified dates to work on annotating sequences and their cumulative work time is recorded. This number is summed for all annotators and the total resulting time is the annotation cost of the sequence. \vspace{-.3cm}}

\label{fig: real_labeling_time}
\end{figure}

\subsection{Dataset Statistics Details}
Within this section, we describe details surrounding key aspects of the dataset that haven't been elaborated in the main paper. 

\subsubsection{Frame Quantity Distribution}
We show the distribution of frame quantity for all sequences in Figure \ref{fig: frame_dist}. The majority of sequences are constrained within 594 to 864 frames, indicating that the sequences contain a relatively equal number of frames. This avoids bias in terms of utilizing sequence length as a major indicator for querying. Ideally, active learning algorithms should utilize the inherent information and difficulties with labeling to achieve high generalization and low annotation cost, instead of querying according to the variation of sequence length. 

\begin{figure*}[h!]
\centering
\includegraphics[scale=.5]{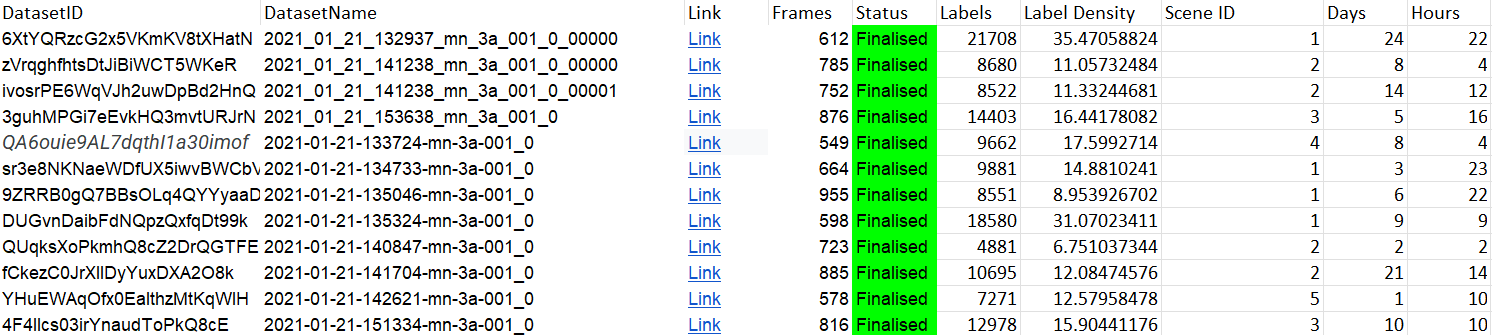}

\caption{Example of how label and cost information is organized within the \texttt{FOCAL} dataset. Every sequence is assigned a cost value based on the time associated with annotating the sequence. \vspace{-.3cm}}

\label{fig: sequence_screenshot}
\end{figure*}

\begin{figure}[h!]
\centering
\includegraphics[scale = .75]{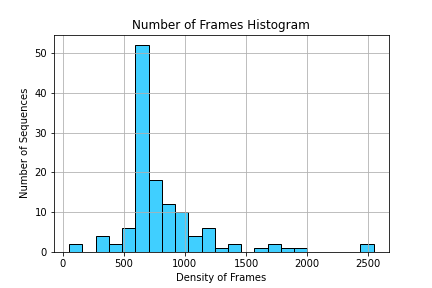}

\caption{Variation of frame quantity in sequences. The majority of collected sequences consist of a relatively equal number of frames. This avoids potential bias in terms of sequence length in querying strategies.\vspace{-.3cm}}

\label{fig: frame_dist}
\end{figure}

\begin{figure}[h!]
\centering
\includegraphics[width = 6in]{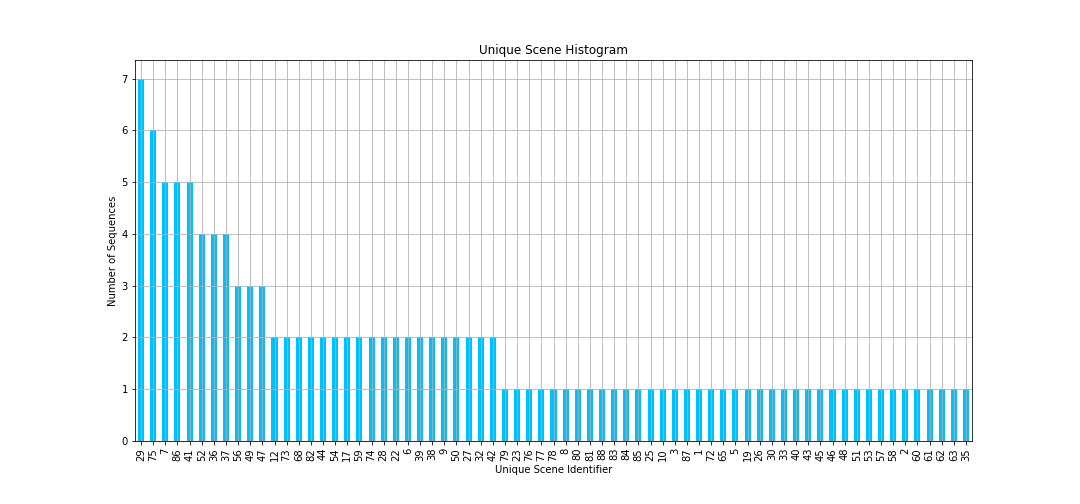}

\caption{Unique scene identities. All sequences are grouped into 69 unique scenes to obtain non-overlapping training and test scenes. The x-axis represents assigned scene identities. The y-axis shows the number of sequences collected at each corresponding scene.\vspace{-.3cm}}

\label{fig: scene_id}
\end{figure}

\begin{figure}[h!]
\centering
\includegraphics[scale=.35]{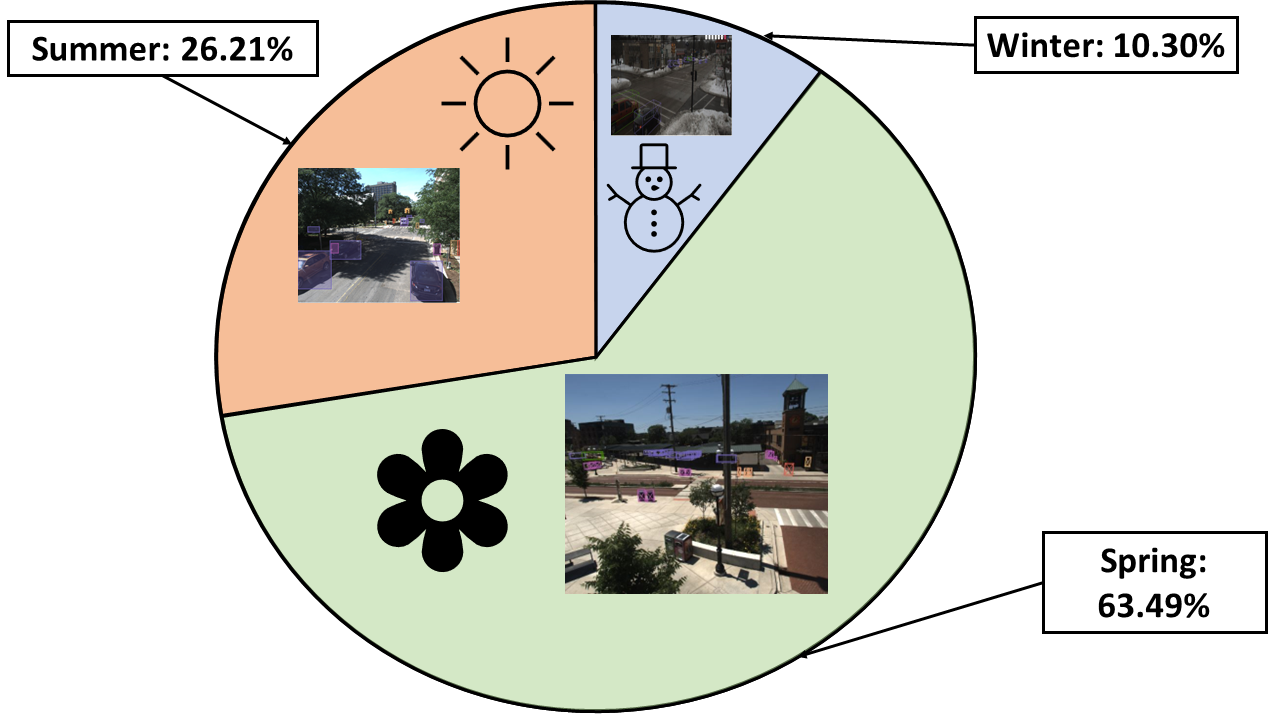}

\caption{Season distribution in the \texttt{FOCAL} dataset. The sequences were collected in multiple seasons to encourage diverse environmental conditions and object activities.\vspace{-.3cm}}

\label{fig: season_pie}
\end{figure}

\begin{figure}[h!]
\centering
\includegraphics[scale = .8]{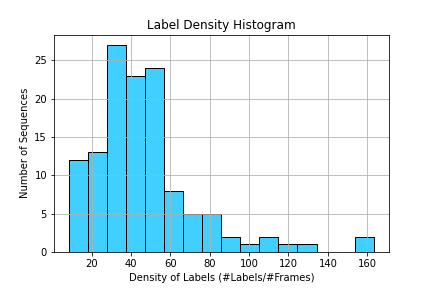}

\caption{Object instance density. Object diversity is presented in the \texttt{FOCAL} dataset.\vspace{-.3cm}}

\label{fig: obj_density}
\end{figure}

\subsubsection{Scene Diversity} In order to obtain training and test sequences in non-overlapping scenes, we manually group all sequences into 69 unique scenes according to their geographic locations. We assign each scene a unique identifier. The sequences collected at the same scene are associated with the same scene identifier. The statistics of scene identities are shown in Figure \ref{fig: scene_id}. In addition to location diversity, sequences in \texttt{FOCAL} also contain varied environmental conditions. For instance, the sequences were collected in multiple seasons, including winter, spring, and summer, as shown in Figure \ref{fig: season_pie}. Overall, there are 41\%, 8\%, and 51\% sequences collected in the winter, spring, and summer, respectively. The variation of these scenes encourages diverse data conditions to evaluate active learning algorithms.

\subsubsection{Object Diversity} In addition to the variation in the scenes, sequences in \texttt{FOCAL} also contains object diversity. Figure \ref{fig: obj_density} illustrates the statistics of averaged object quantity per frame across all sequences. Due to the variation in locations and environmental conditions, the number of object instances varies across different sequences. This object density variation is beneficial to the evaluation of active learning algorithms. 

\subsubsection{Change of Object Quantity}
The temporal first-order statistics of the accumulative object quantity can be considered as a factor of annotation cost. Specifically, we calculate such statistics as the change of object quantity between a certain fixed number of frames, as shown in Fig~\ref{fig: change_objquant}. A higher number of mobile objects moving in and out of the field of view can result in higher annotation costs due to more efforts in accurately tracking these objects.

% \subsubsection{Occlusion Statistics}
% There are different levels of object-wise occlusion severity, i.e. partially visible, fully occluded, and visible, in the annotations. 

% In addition, there exist variations in the occlusion severity due to the motion of objects. In order to represent the overall occlusion severity of each sequence, we calculate the weighted sum of object-wise occlusion severity as $(0.5\times$  \# partially visible $+ 1\times$ \# fully occluded $+ 0.2\times$ \# visible$)$ as shown in Fig~\ref{fig: weighted_occlusion}. It is likely to take higher annotation costs due to more occluded objects and/or higher levels of severity. 

\begin{figure}[h!]
\centering
\includegraphics[scale=0.7]{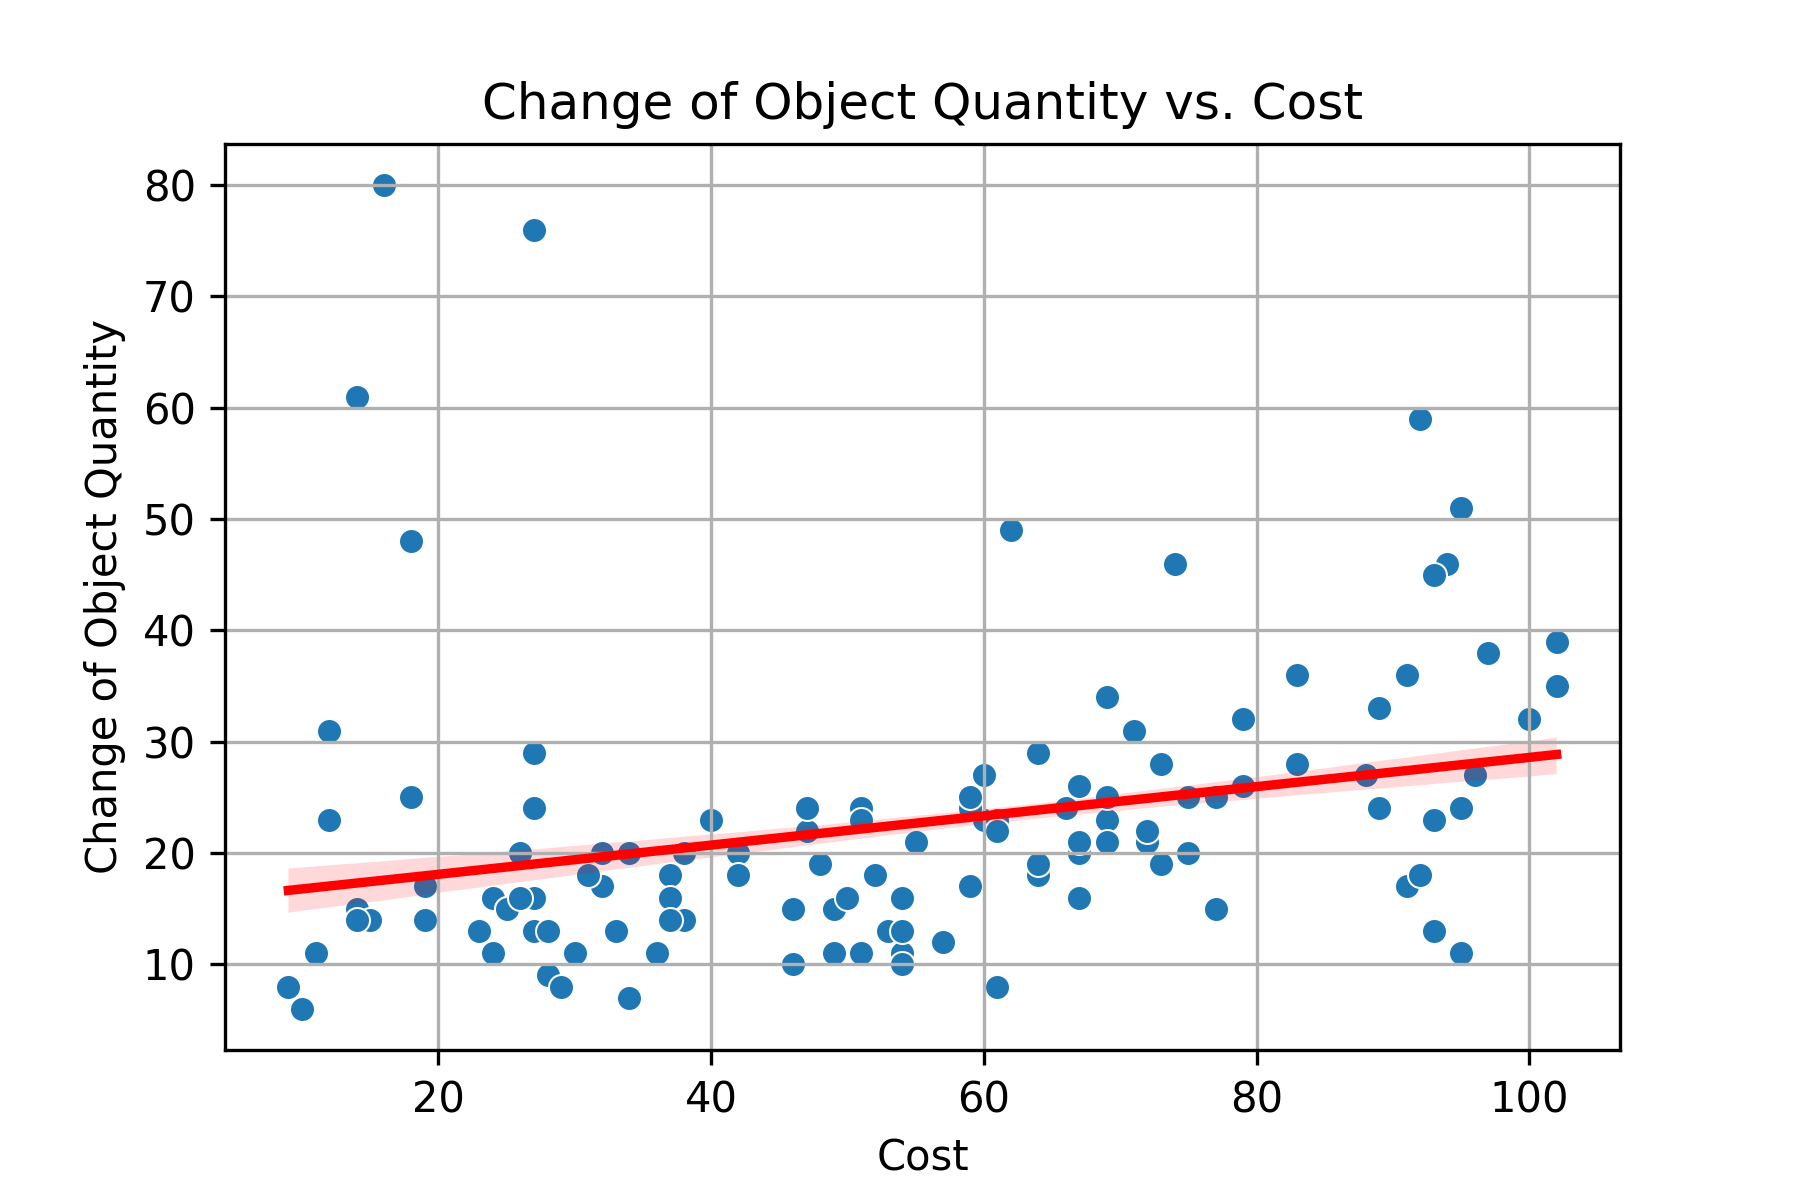}

\caption{Change of object quantity.\vspace{-.3cm}}

\label{fig: change_objquant}
\end{figure}

\begin{figure}[h!]
\centering
\includegraphics[scale=0.7]{Fig/cost_analysis/WEIGHTED OCCLUSION vs. Total Cost.png}

\caption{Statistics of object-wise weighted occlusion.\vspace{-.3cm}}

\label{fig: weighted_occlusion}
\end{figure}

\begin{figure}[h!]
\centering
\includegraphics[width = \columnwidth]{Fig/Van Images/van_details.png}

\caption{Layout of data collection setup for van.\vspace{-.3cm}}

\label{fig: van_details}
\end{figure}

\begin{figure}[h!]
\centering
\includegraphics[width = \columnwidth]{Fig/Van Images/van_interior.pdf}

\caption{Interior setup for the van.\vspace{-.3cm}}

\label{fig: van_interior}
\end{figure}

\begin{figure}[h!]
\centering
\includegraphics[width = \columnwidth]{Fig/Van Images/sensor_layout.png}

\caption{Sensor layout of cameras and lidar used for data collection.\vspace{-.3cm}}

\label{fig: sensor layout}
\end{figure}

\subsection{Experimental Setup: Relationship Between Estimated Motion and Estimated Boxes with Cost}
\begin{figure} [h!]
\centering
\includegraphics[width=\textwidth]{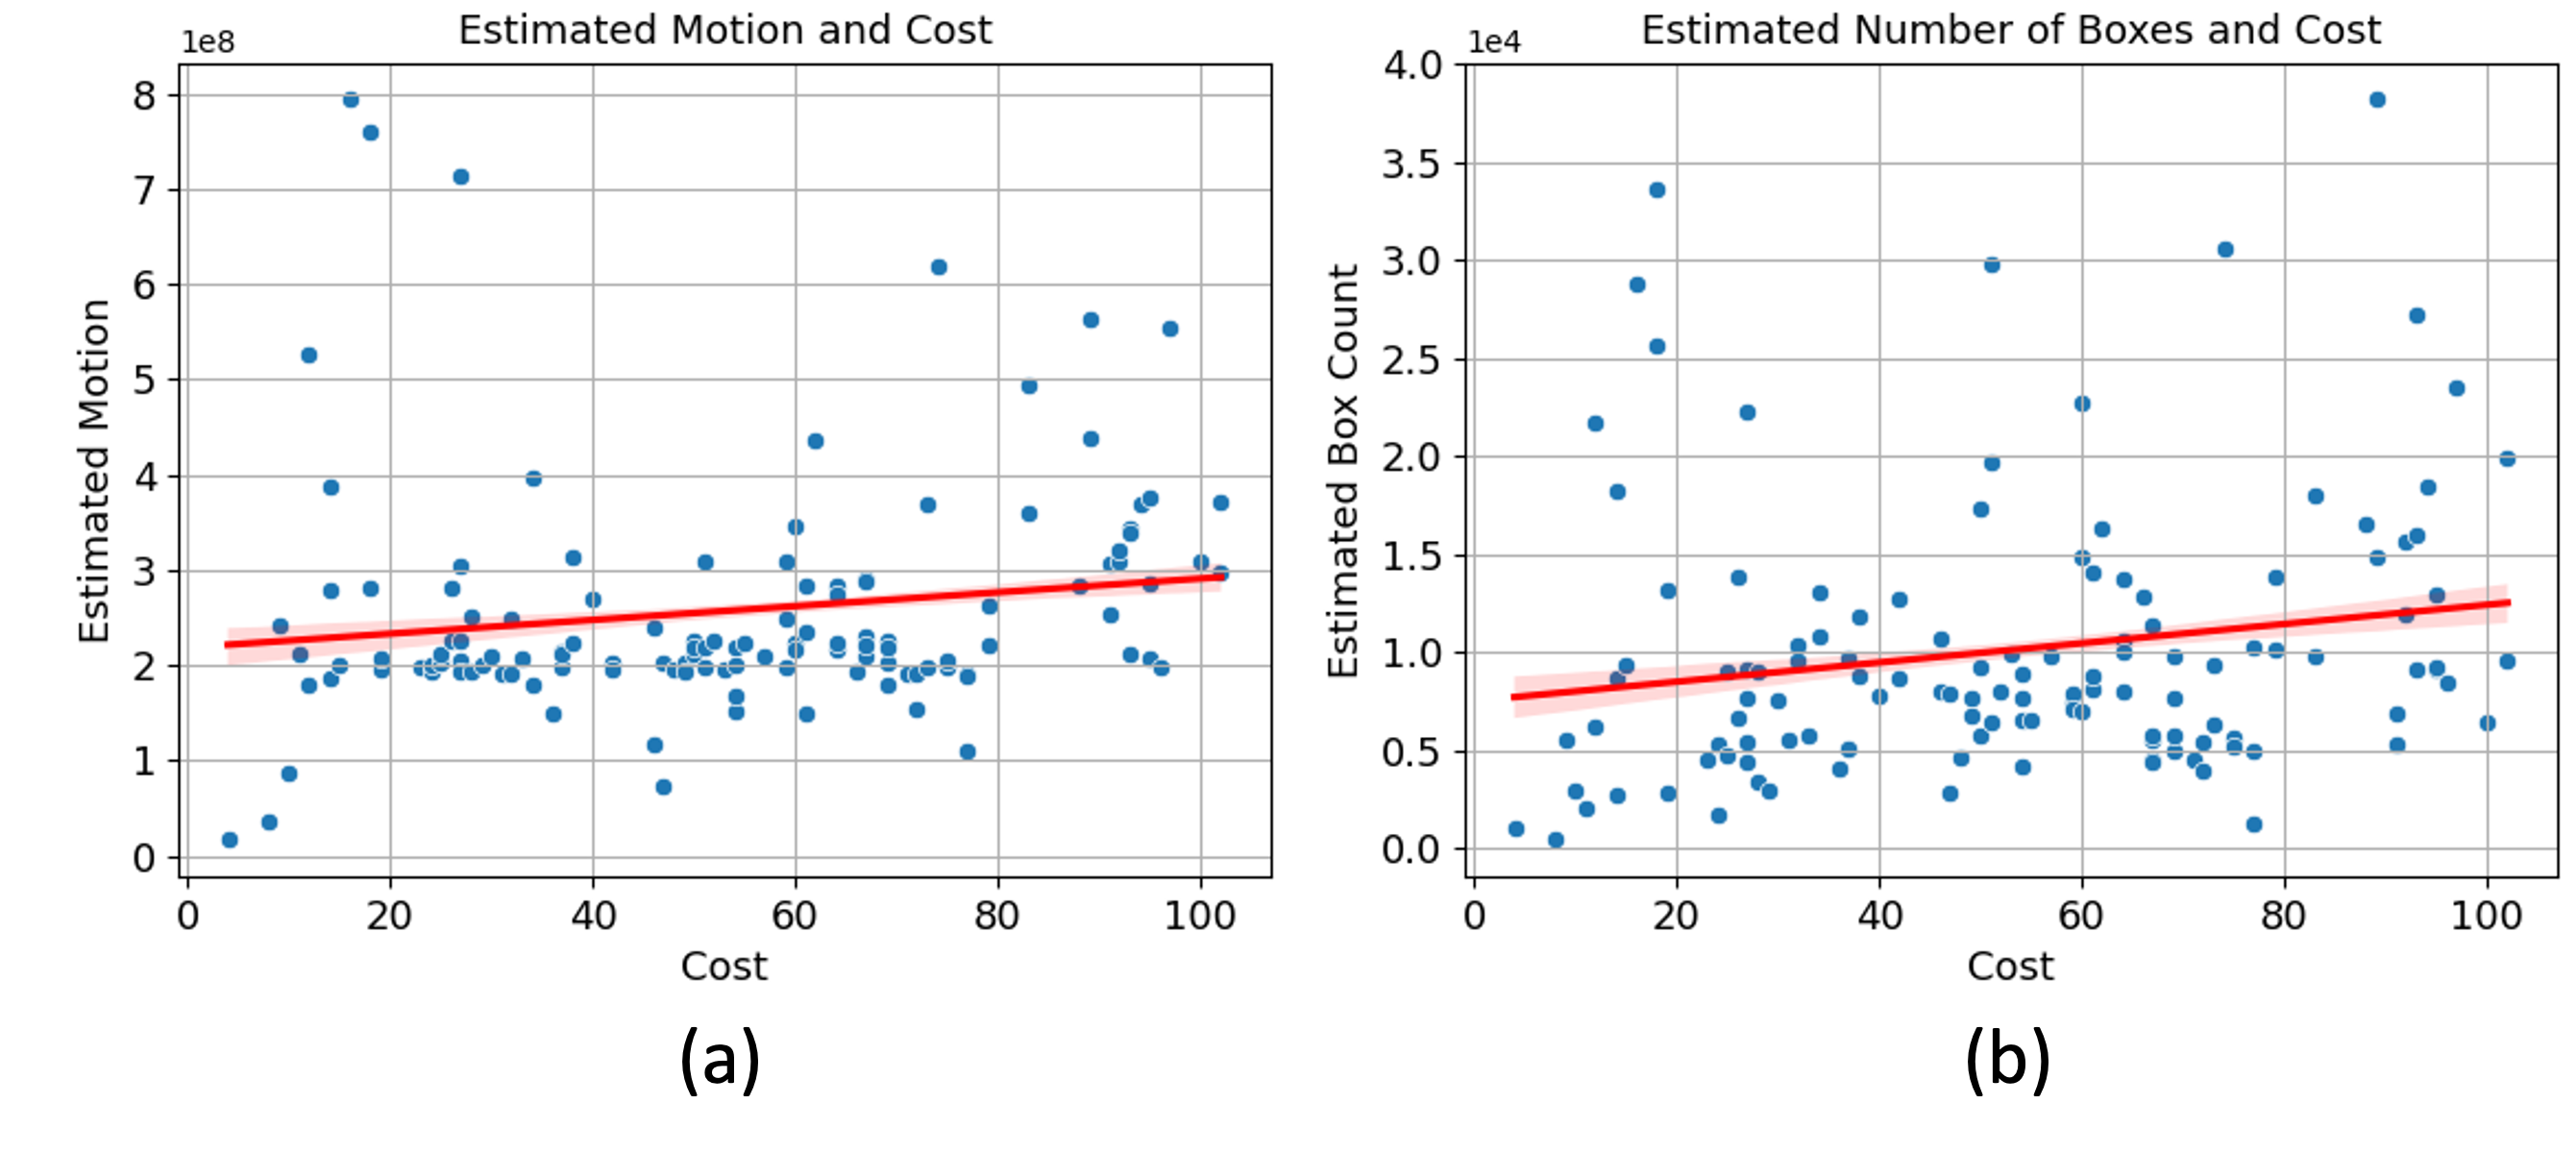}
\caption{(a) The relationship between estimated motion (derived from optical flow) and cost. (b) The relationship between estimated box count (also derived from optical flow) and cost.}
\label{fig:est_queries}
\end{figure} 

\subsection{Smart City Van}
\subsubsection{Motivation}
The smart infrastructure node (smart IX node) was developed to provide a stationary sensing platform that can be deployed in environments where smart vehicles can utilize additional information from an infrastructure perspective to aid in navigating the world around them. When we started to develop algorithms to run on these nodes, we lacked a lot of the standard data that was widely available for autonomous vehicles since this was a new area of work. Namely, we needed annotated data that was representative of an infrastructure perspective, the ability to test and experiment with new sensors at a multitude of public locations, and the ability to experiment with and examine the effects of sensor placement in real-time. 

\subsubsection{Approach}

Since the cost to install these sensors is high, it would have been impossible to install these IX nodes in enough locations to cover all possible weather conditions, times of day, and even types of objects that we could see from an IX node. For autonomous vehicles, this is relatively easy because the vehicle can be driven through any type of environment, weather condition, or location in order to collect representative data that could be used for training. For the IX, this is not as easy, since the platform is stationary. Furthermore, collecting large amounts of data from a limited set of IX nodes with fixed points of view could cause model overfitting to the stationary context (e.g., background) that we captured from these few nodes. We needed something more mobile so that the data can cover various viewpoints, orientations, and locations. 

To achieve a more mobile data collection process, we could have used a similar sensor mount as on the IX and placed it on a tripod that can be moved and set up at any location. This was feasible but it would not have been easy to move around, set up, power, and collect data from different locations.

The mobile van solution provided us the best of both worlds by supplying the same sensor setup as the IX nodes (with the option for testing other sensors as well) along with the mobility of a tripod that's easier to use and collect data from.

\subsubsection{Van Details}
The smart city van was custom built with our internal transit team. The sensors are mounted on the outside on a telescoping mast with pan and tilt controls, providing 360 degrees of horizontal and vertical rotation. The mast can be extended from 6ft to 20 ft. When combined with the vehicle's height, that provides a height range of 16 ft up to 30 ft. There is also a roof mount AC that was used to cool the interior space as well as the inside electronics. To power all of this, there is a 7.5kW Diesel generator (which shared the fuel tank with the vehicle) on board to provide ample power no matter where the vehicle goes. There is also an option to use power from a standard 120V 15 or 30A outlet when testing in a garage. All of these are detailed in Figure \ref{fig: van_details}.

The interior of the shuttle, visualized in Figure \ref{fig: van_interior}, provides controls for raising, lowering, and adjusting the mast from within the vehicle as well as two workstations to be able to monitor and collect data, all without getting out of the van. The workstations have a 4G modem/router to provide wired and Wi-Fi connectivity and there is a server rack for easily connecting and removing hard disks from the onboard computer. Furthermore, there is an alarm to warn if the vehicle goes out of the park while the mast is still raised. There is also an electronics panel with controls for the AC system, DC/battery system, and the generator. On top of the mast is the sensor setup with the camera system utilized for data collection in Figure \ref{fig: sensor layout}. 

%Power Panel: DC Power Panel (RED) controls the vehicle's 12V DC power system. Currently, the only electronics on the DC system are the interior lights.  AC Power Panel (Green) controls the vehicle's AC power system. There are two possible sources of AC power, the shore line, and the generator. Only one AC power source can be used at a time. Most equipment in the van runs on the AC system, this includes all rack and interior power receptacles, the air conditioner, and the AC/DC converter.  Generator Control (BLUE) is the start/stop button for the generator. It also contains the time running time for the generator.  DC Panel Physical Disconnect (ORANGE) switch controls a physical disconnect between the battery/source and the 12V DC system. This is used to prevent the drain on the 12V battery when the vehicle is not in use.

\subsection{Cost Analysis with Modern Annotation Optimizations}
\label{sec:appendix-cost-analysis}
In our cost analysis, we simulate modern annotation software for sequential approaches. Specifically, we estimate singular cost under the assumption of label interpolation and perform experiments with different interpolation rates. We show an example of label interpolation with ten frames of the same \texttt{FOCAL} sequence in Figure~\ref{fig:interpolation-toy}. Instead of annotating every single frame, temporal dependencies can be utilized to interpolate object labels in between two fully annotated frames at nearly zero cost. While static objects result in a simple label copy, dynamic object labels are interpolated through linear mappings as shown in the bottom half of the figure. In this example, we are assuming an interpolation rate of ten - i.e. only every tenth frame is fully annotated. Since the interpolation rate is not static in practical scenarios, we only consider conservative interpolation rates (five, two, and no interpolation).
% Add details about explicit implementations of different strategies here.
\begin{figure}[h!]
	\centering
	\includegraphics[width = \columnwidth]{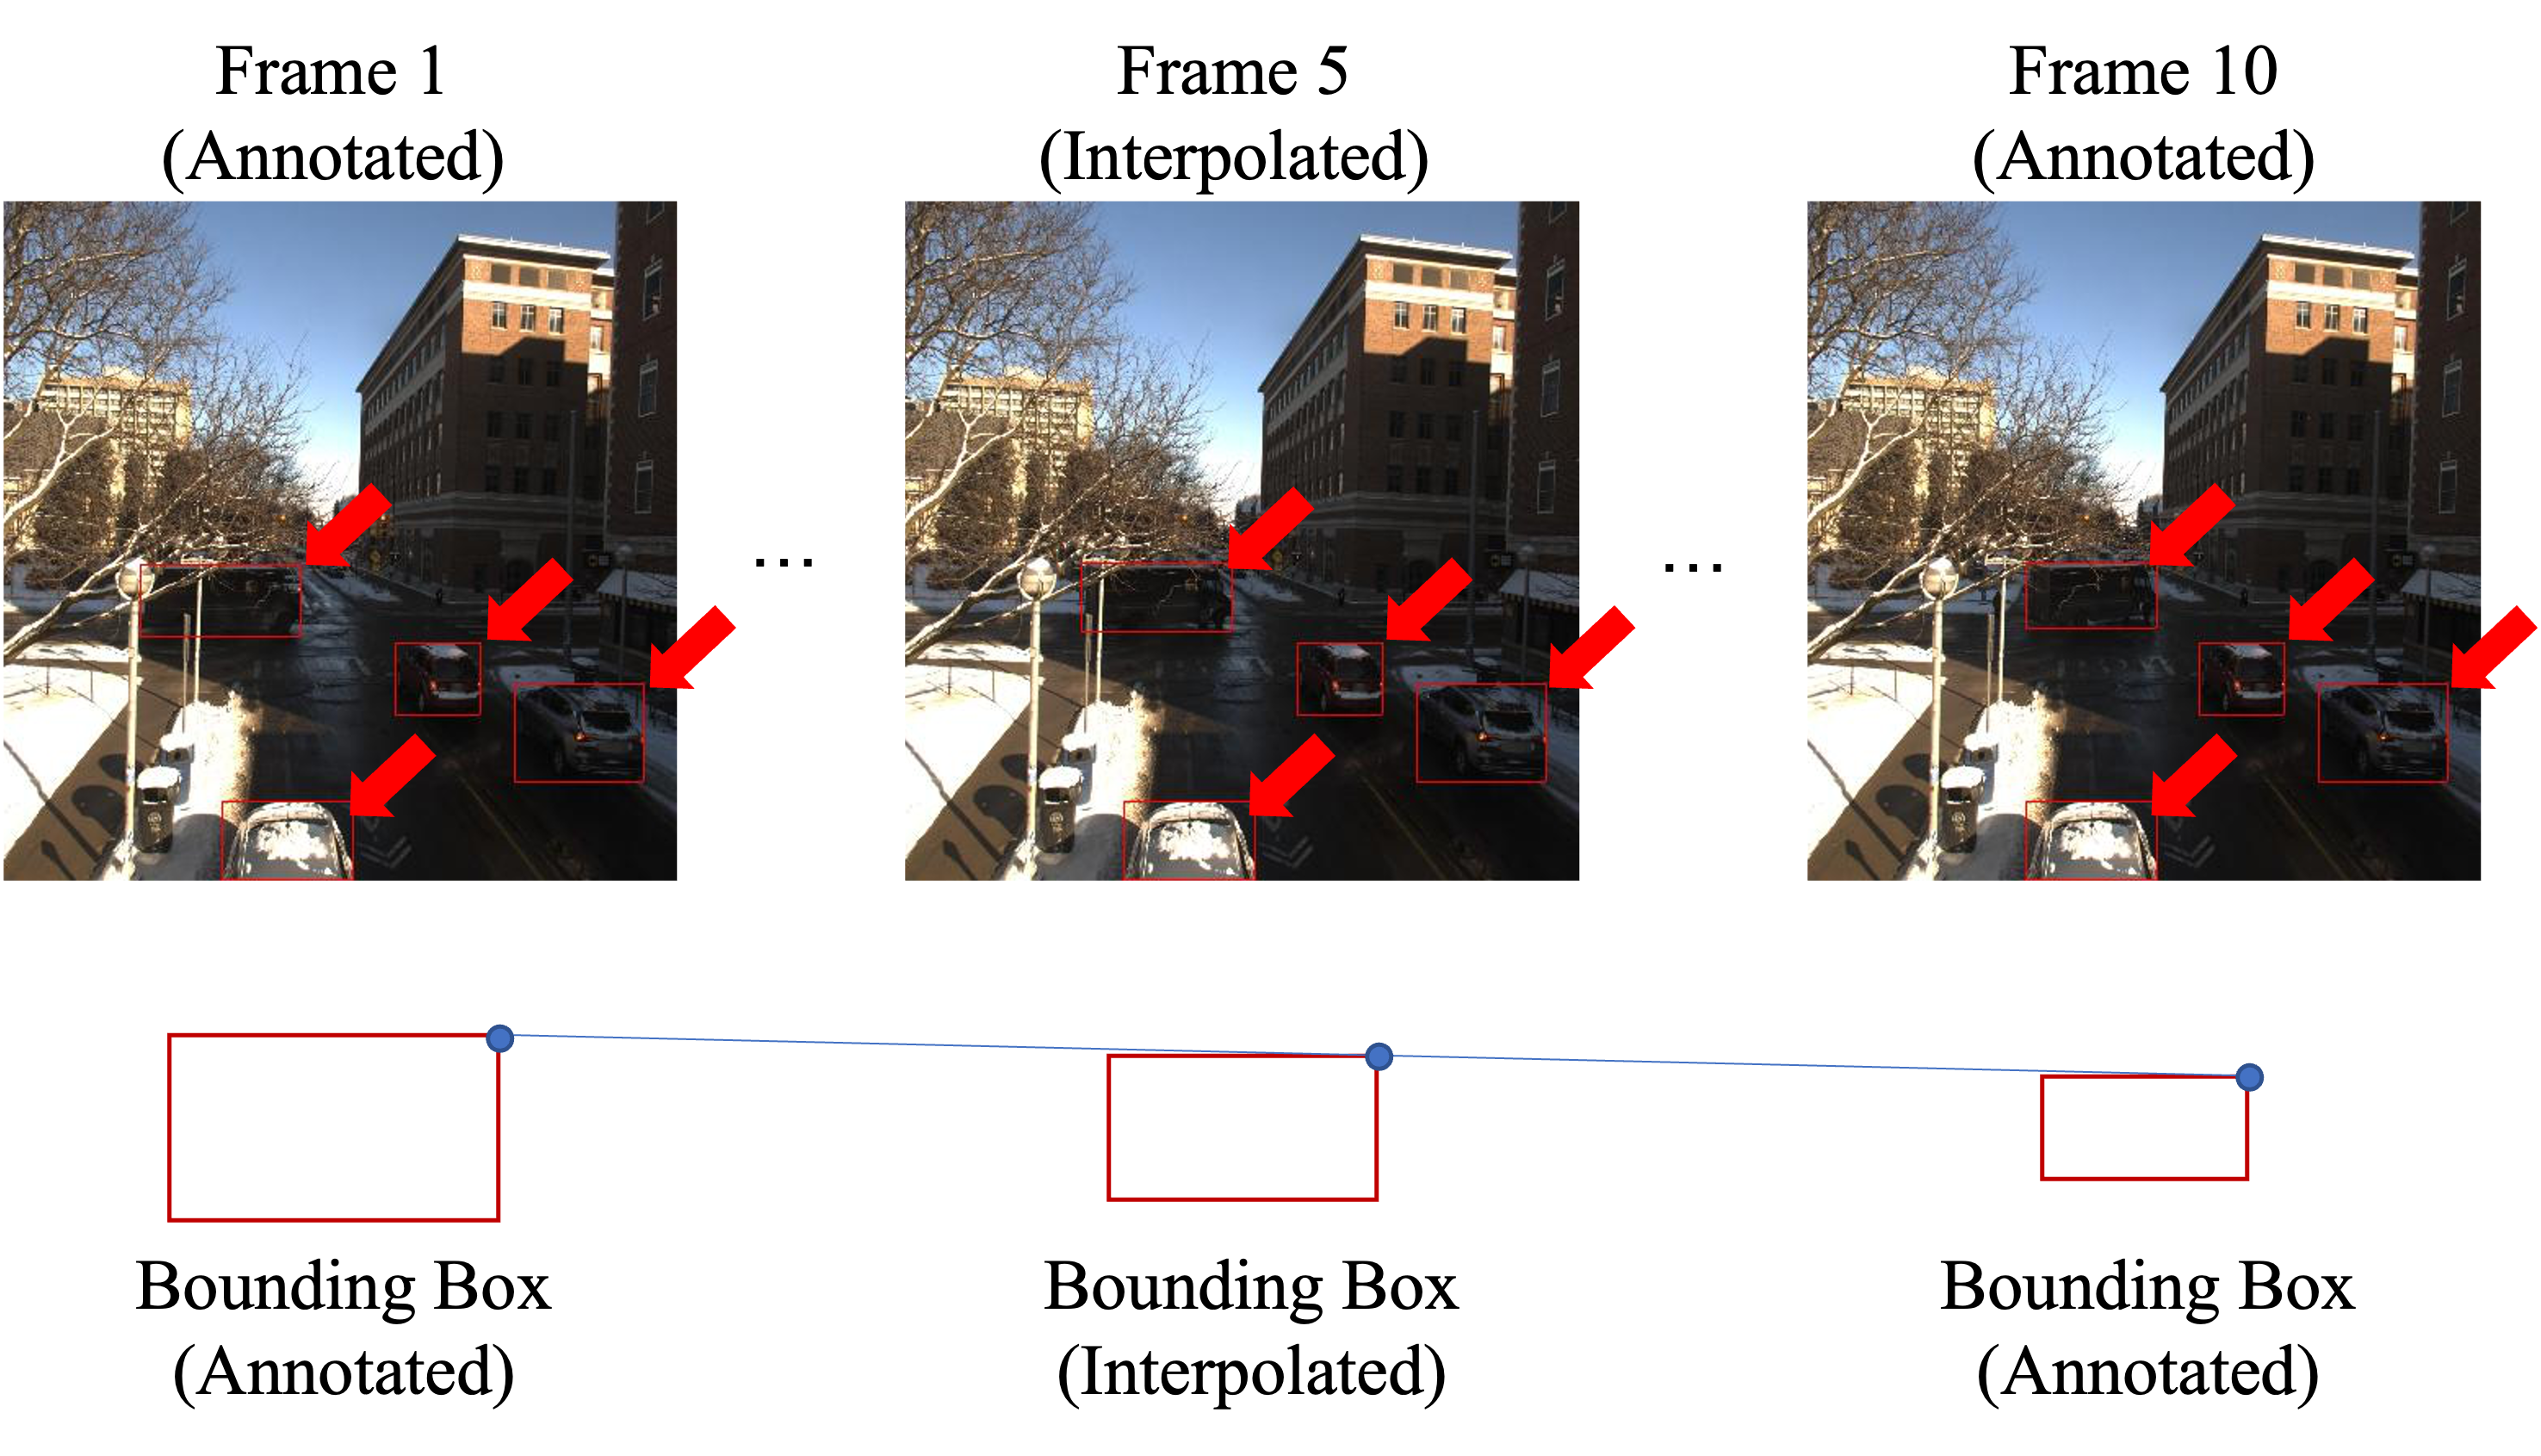}
	
	\caption{Label interpolation on a \texttt{FOCAL} sequence. Instead of annotating all objects in every frame, the annotator annotates Frame~1 and Frame~10 and interpolates the remaining labels. For interpolation, a simple linear mapping is used (bottom half).}
	
	\label{fig:interpolation-toy}
\end{figure}

\begin{figure*}[h!]
\centering
\includegraphics[width=\textwidth]{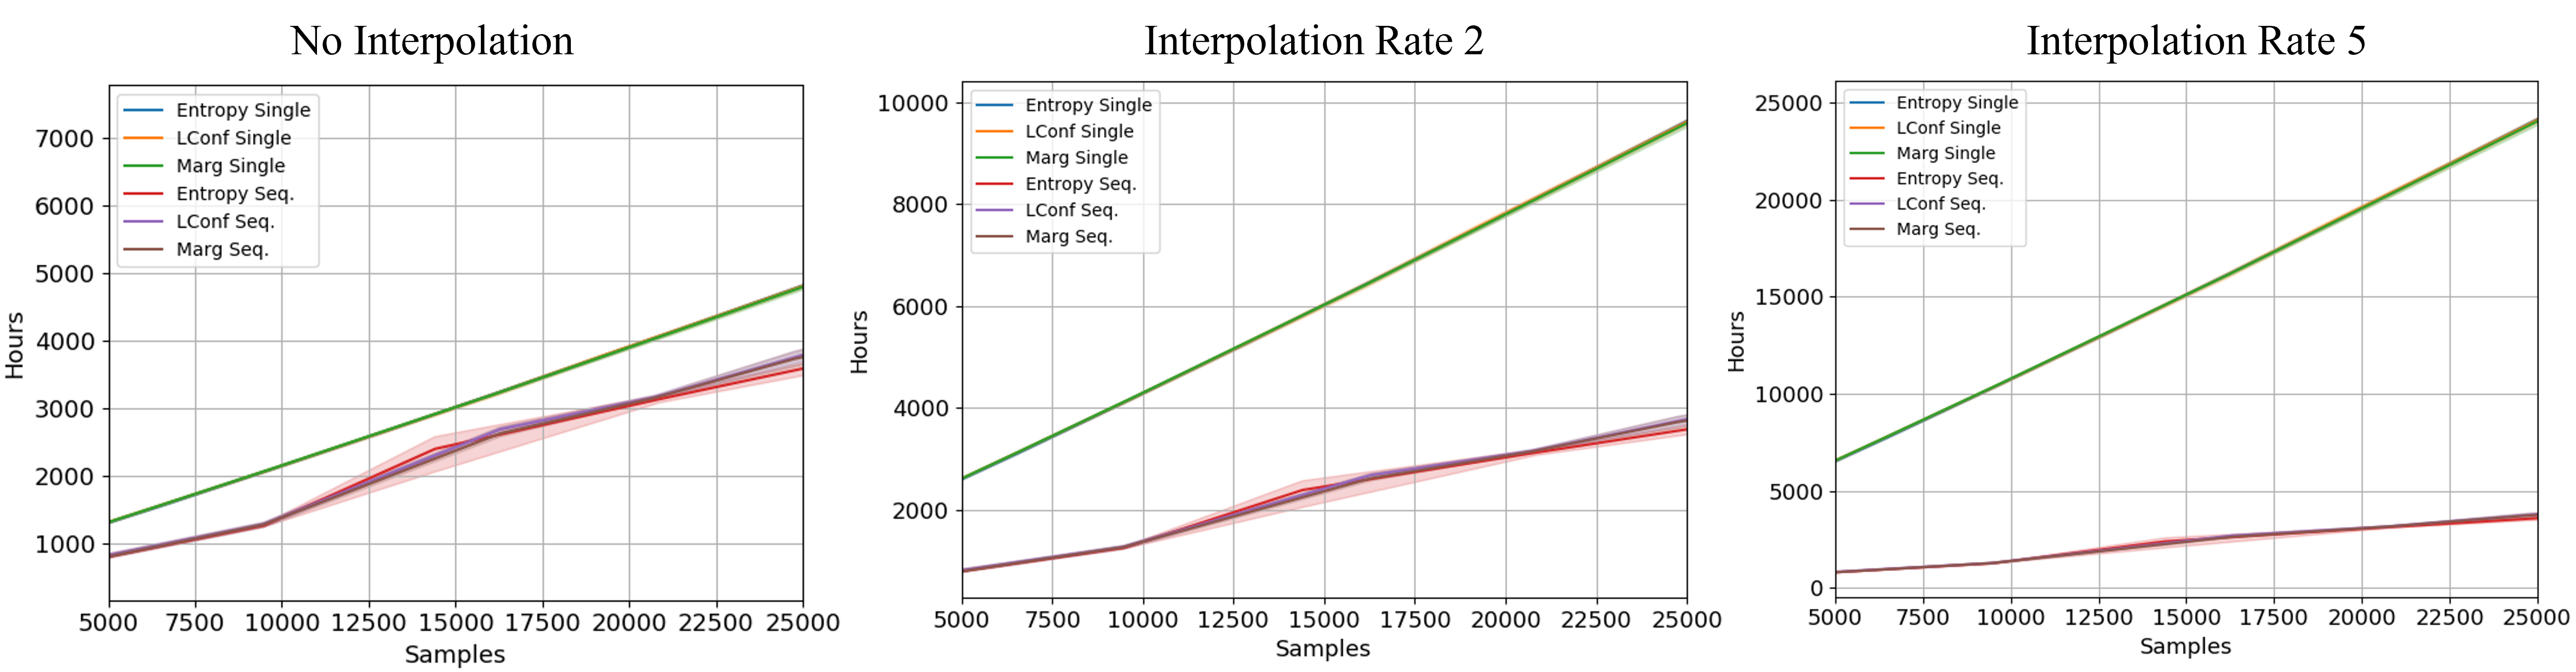}

\caption{Cost of sequential and single frame entropy sampling, margin sampling, and least confidence sampling on the \texttt{FOCAL} dataset when assuming different interpolation rates. Left: no interpolation. Middle: every second frame in sequence is annotated (rest interpolated). Right: every fifth frame in sequence is annotated (rest interpolated).}
\label{fig:cost-single-seq}
\end{figure*}
We use the same experimental setup as in the main paper. In order to derive the cost of annotating single frames, we divide the total sequence cost by the effectively annotated frames assuming a fixed frame interpolation rate. For instance, a sequence of 100 sequentially correlated frames can be fully labeled by annotating every 10th frame in detail and interpolating the remaining frames with zero cost. Assuming the entire sequence took 10h to label, the cost-per-frame would be 1h (10h / 10 effective frames). We show the cost in hours for entropy sampling, margin sampling, and least confidence sampling with two, and five respectively (Figure~\ref{fig:cost-single-seq}). For a fair comparison, we additionally include our results with no interpolation that are discussed in the main paper. Complimentary to our previous observations, sequential approaches consistently outperform singular strategies regardless of the interpolation rate.
