# Supplementary material for: FOCAL: A Cost-Aware Video Dataset for Active Learning
Source: arXiv:2311.10591 source file (2023-11-17)
Supplement: Supplementary file 5 [file AppendixB.tex]

\subsection{Dataset Curation} \label{app:curation}

The sequential video data was collected via stationary cameras mounted on a vehicle at various locations across primarily Ann Arbor and Detroit Michigan from January 2021 to August 2021. Examples of locations where videos were recorded can be found in Figure \ref{fig:map}. This was accomplished through the use of the Smart City Van as further described in section \ref{app:smart_van}. On top of the van is an adjustable rig that mounts the camera for video sequence acquisition. The camera used is a FLIR BlackFlyS camera with a 6mm lens mounted on a locking telescopic mast installed on the roof of a van. The raw images are at a 5MP (mega-pixel) resolution, while the resolution of the undistorted images varies slightly due to the variation of the undistortion parameters.

\begin{figure} [t!]
\centering
\includegraphics[width=\columnwidth]{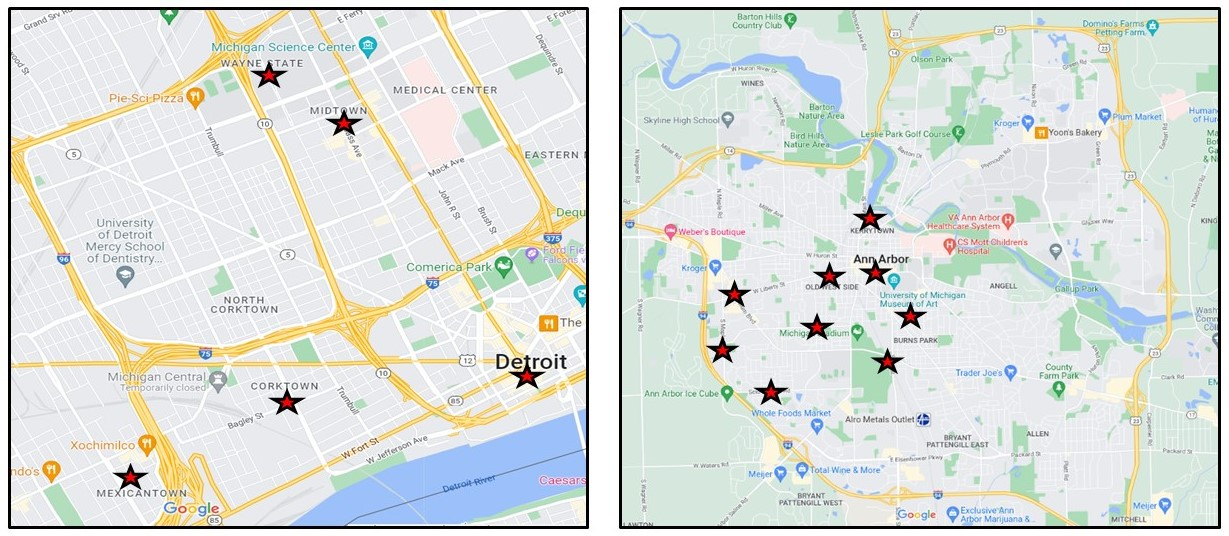}
\caption{Examples of of a variety of locations where data collection was performed for the FOCAL dataset.}
\label{fig:map}
\end{figure} 

\subsection{Labeling Details} \label{app:labeling}

Within this section, we show specific details surrounding the labeling process. After the data is entered into the online annotation platform, the annotator uses the setup shown in Figure \ref{fig: real_labeling} in order to assign bounding boxes to the objects in the scene as well as interpolate these objects across the sequence.
Also within this annotation tool is a system to track the amount of time each user spends working on a sequence. This is shown through the example for a specific sequence in Figure \ref{fig: real_labeling_time}. The x-axis shows the dates on which the work on the sequence was performed and the y-axis indicates the number of cumulative hours across all users for that specific sequence. The labeling work is divided into quality assurance and annotation time. 
%% added Armin's comments here.
The potential annotation bias is reduced by allocating separate objects across the entire sequence, instead of assigning frames, to different annotators. Specifically, each annotator annotates one object throughout the entire sequence,  then goes back to the beginning of the sequence and takes another object to assign labels. After annotations were completed for an individual sequence, the sequence was sent for review to a separate team who performed quality assurance for the curated annotations. The quality assurance  ensures that we achieve above 95\% accuracy during the labeling process, where the accuracy is calculated as 1 - (missed annotations + incorrect classifications + incorrect attributes + false annotation) / total number of objects labeled. If the accuracy goes lower than 95\%, the sequence needs to be annotated from scratch by the supplier.
For the annotation time cost, the sum of all hours worked on each date is the final labeling time for the sequence. Figure \ref{fig: sequence_screenshot} shows how every sequence comes with its own identity as well as information regarding frames, the quantity of bounding boxes, unique scene identifier, and the cumulative number of days and hours it took to label the sequence. Participants who annotated the data and performed quality assurance were compensated appropriately for their services.

\begin{figure}[h!]
\centering
\includegraphics[width = \columnwidth]{Fig/Van Images/labeling.png}

\caption{Example of labeling setup within our internal platform.\vspace{-.3cm}}

\label{fig: real_labeling}
\end{figure}

\begin{figure}[h!]
\centering
\includegraphics[width = \columnwidth]{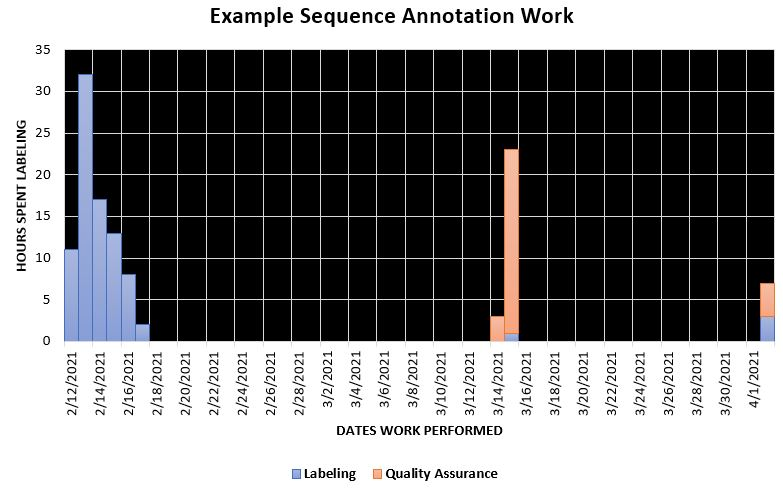}

\caption{Example of how cost annotation is calculated within the labeling tool. Users log in on specified dates to work on annotating sequences and their cumulative work time is recorded. This number is summed for all annotators and the total resulting time is the annotation cost of the sequence. \vspace{-.3cm}}

\label{fig: real_labeling_time}
\end{figure}

\begin{figure*}[h!]
\centering
\includegraphics[scale=.5]{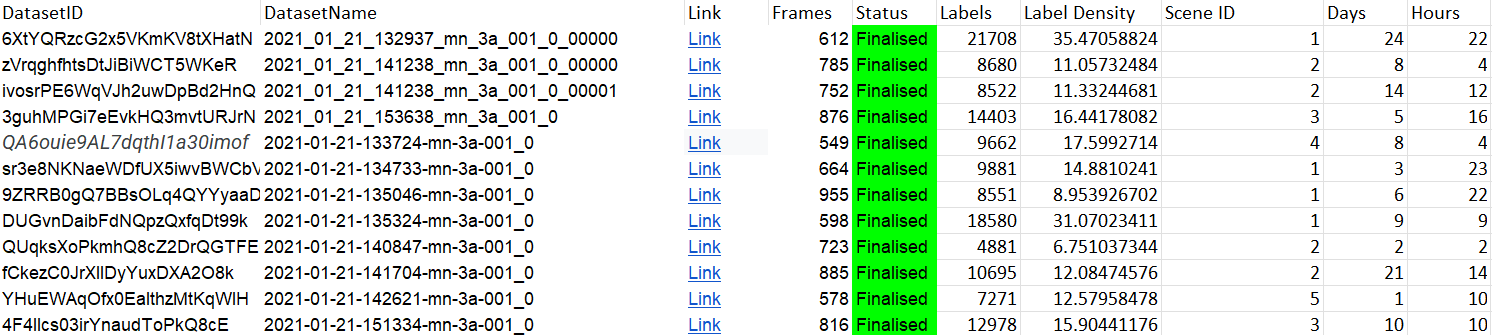}

\caption{Example of how label and cost information is organized within the \texttt{FOCAL} dataset. Every sequence is assigned a cost value based on the time associated with annotating the sequence. \vspace{-.3cm}}

\label{fig: sequence_screenshot}
\end{figure*}

\subsection{Cost Acquisition} \label{app:cost_acquisition}

In Figure \ref{fig: cost_comp}, we provide a detailed overview of how we obtained the cost label for every sequence. First, videos are received as raw data from the cameras used on the Smart City Van. This raw video data is passed to the annotators at an associated labeling company. While annotating the sequence for the presence of various objects, a timing mechanism monitors their activity to measure how much time is spent interacting with the tool. This value across all users that perform annotation is accumulated as the total annotation time. Once annotation is complete, the sequence is passed to a team that performs customer quality assurance on the sequence for any discrepancies or errors that accumulated during labeling. This results in an associated time that is added to the overall cost. The final step is a final review where the sequence is approved for entry into the dataset. The total cost across all three of these steps is what constitutes the final cost label for the sequence. 

\begin{figure}[h!]
\centering
\includegraphics[width = \columnwidth]{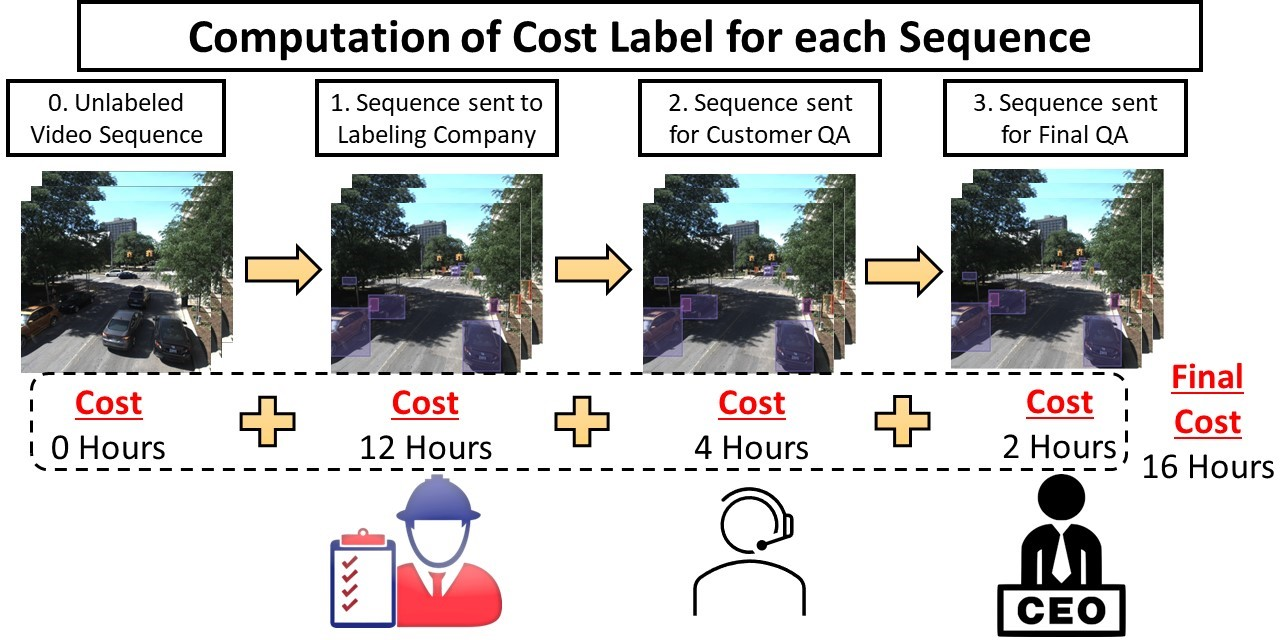}

\caption{This is the process by which cost is computed. 0) The raw video stream is received. 1) Time for all annotators to complete labeling is recorded. 2) The labeled sequence is sent to a customer quality assurance team. This assurance time is recorded. 3) The final step is a final review of the sequence and the cost for each one of these steps is accumulated to contribute to the final cost label of the sequence. \vspace{-.3cm}}

\label{fig: cost_comp}
\end{figure}

\subsection{Smart City Van} \label{app:smart_van}
\subsubsection{Motivation}
The smart infrastructure node (smart IX node) was developed to provide a stationary sensing platform that can be deployed in environments where smart vehicles can utilize additional information from an infrastructure perspective to aid in navigating the world around them. When we started to develop algorithms to run on these nodes, we lacked a lot of the standard data that was widely available for autonomous vehicles since this was a new area of work. Namely, we needed annotated data that was representative of an infrastructure perspective, the ability to test and experiment with new sensors at a multitude of public locations, and the ability to experiment with and examine the effects of sensor placement in real-time. 

\subsubsection{Approach}

Since the cost to install these sensors is high, it would have been impossible to install these smart infrastructure (IX) nodes in enough locations to cover all possible weather conditions, times of day, and even types of objects that we could see from an IX node. For autonomous vehicles, this is relatively easy because the vehicle can be driven through any type of environment, weather condition, or location in order to collect representative data that could be used for training. For the IX, this is not as easy, since the platform is stationary. Furthermore, collecting large amounts of data from a limited set of IX nodes with fixed points of view could cause model overfitting to the stationary context (e.g., background) that we captured from these few nodes. We needed something more mobile so that the data can cover various viewpoints, orientations, and locations. 

To achieve a more mobile data collection process, we could have used a similar sensor mount as on the IX and placed it on a tripod that can be moved and set up at any location. This was feasible but it would not have been easy to move around, set up, power, and collect data from different locations.

The mobile van solution provided us the best of both worlds by supplying the same sensor setup as the IX nodes (with the option for testing other sensors as well) along with the mobility of a tripod that's easier to use and collect data from.

\begin{figure}[h!]
\centering
\includegraphics[width = \columnwidth]{Fig/Van Images/van_details.png}

\caption{Layout of data collection setup for van.\vspace{-.3cm}}

\label{fig: van_details}
\end{figure}

\begin{figure}[h!]
\centering
\includegraphics[width = \columnwidth]{Fig/Van Images/van_interior.pdf}

\caption{Interior setup for the van.\vspace{-.3cm}}

\label{fig: van_interior}
\end{figure}

\begin{figure}[h!]
\centering
\includegraphics[width = \columnwidth]{Fig/Van Images/sensor_layout.png}

\caption{Sensor layout of cameras and lidar used for data collection.\vspace{-.3cm}}

\label{fig: sensor layout}
\end{figure}

\subsubsection{Van Details}
The smart city van was custom-built with our internal transit team. The sensors are mounted on the outside on a telescoping mast with pan and tilt controls, providing 360 degrees of horizontal rotation and around 60 degrees of vertical rotation. The mast can be extended from 6ft to 20 ft. When combined with the vehicle's height, that provides a height range of 16 ft up to 30 ft. There is also a roof mount AC that was used to cool the interior space as well as the inside electronics, which was used for data collection and live processing. To power all of this, there is a 7.5kW Diesel generator (which shared the fuel tank with the vehicle) on board to provide ample power no matter where the vehicle goes. There is also an option to use power from a standard 120V 15 or 30A outlet when testing in a garage. All of these are detailed in Figure \ref{fig: van_details}.

The interior of the vehicle, visualized in Figure \ref{fig: van_interior}, provides controls for raising, lowering, and adjusting the mast from within the vehicle as well as two workstations to be able to monitor and collect data, all without getting out of the van. The workstations have a 4G modem/router to provide wired and Wi-Fi connectivity and there is a server rack for easily connecting and removing hard disks from the onboard computer. Furthermore, there is an alarm to warn if the vehicle goes out of the park while the mast is still raised. There is also an electronics panel with controls for the AC system, DC/battery system, and generator. On top of the mast is the sensor setup with the camera system utilized for data collection in Figure \ref{fig: sensor layout}.
