# Supplementary material for: FOCAL: A Cost-Aware Video Dataset for Active Learning
Source: arXiv:2311.10591 source file (2023-11-17)
Supplement: Supplementary file 6 [file additionalcostanalysis.tex]

\subsection{Cost Analysis with Modern Annotation Optimizations}
\label{sec:appendix-cost-analysis}
In our cost analysis, we simulate modern annotation software for sequential approaches. Specifically, we estimate singular cost under the assumption of label interpolation and perform experiments with different interpolation rates. We show an example of label interpolation with ten frames of the same FOCAL sequence in Figure~\ref{fig:interpolation-toy}. Instead of annotating every single frame, temporal dependencies can be utilized to interpolate object labels in between two fully annotated frames at nearly zero cost. While static objects result in a simple label copy, dynamic object labels are interpolated through linear mappings as shown in the bottom half of the figure. In this example, we are assuming an interpolation rate of ten - i.e. only every tenth frame is fully annotated. Since the interpolation rate is not static in practical scenarios, we only consider conservative interpolation rates (five, two, and no interpolation).
% Add details about explicit implementations of different strategies here.
\begin{figure}[h]
	\centering
	\includegraphics[width = \columnwidth]{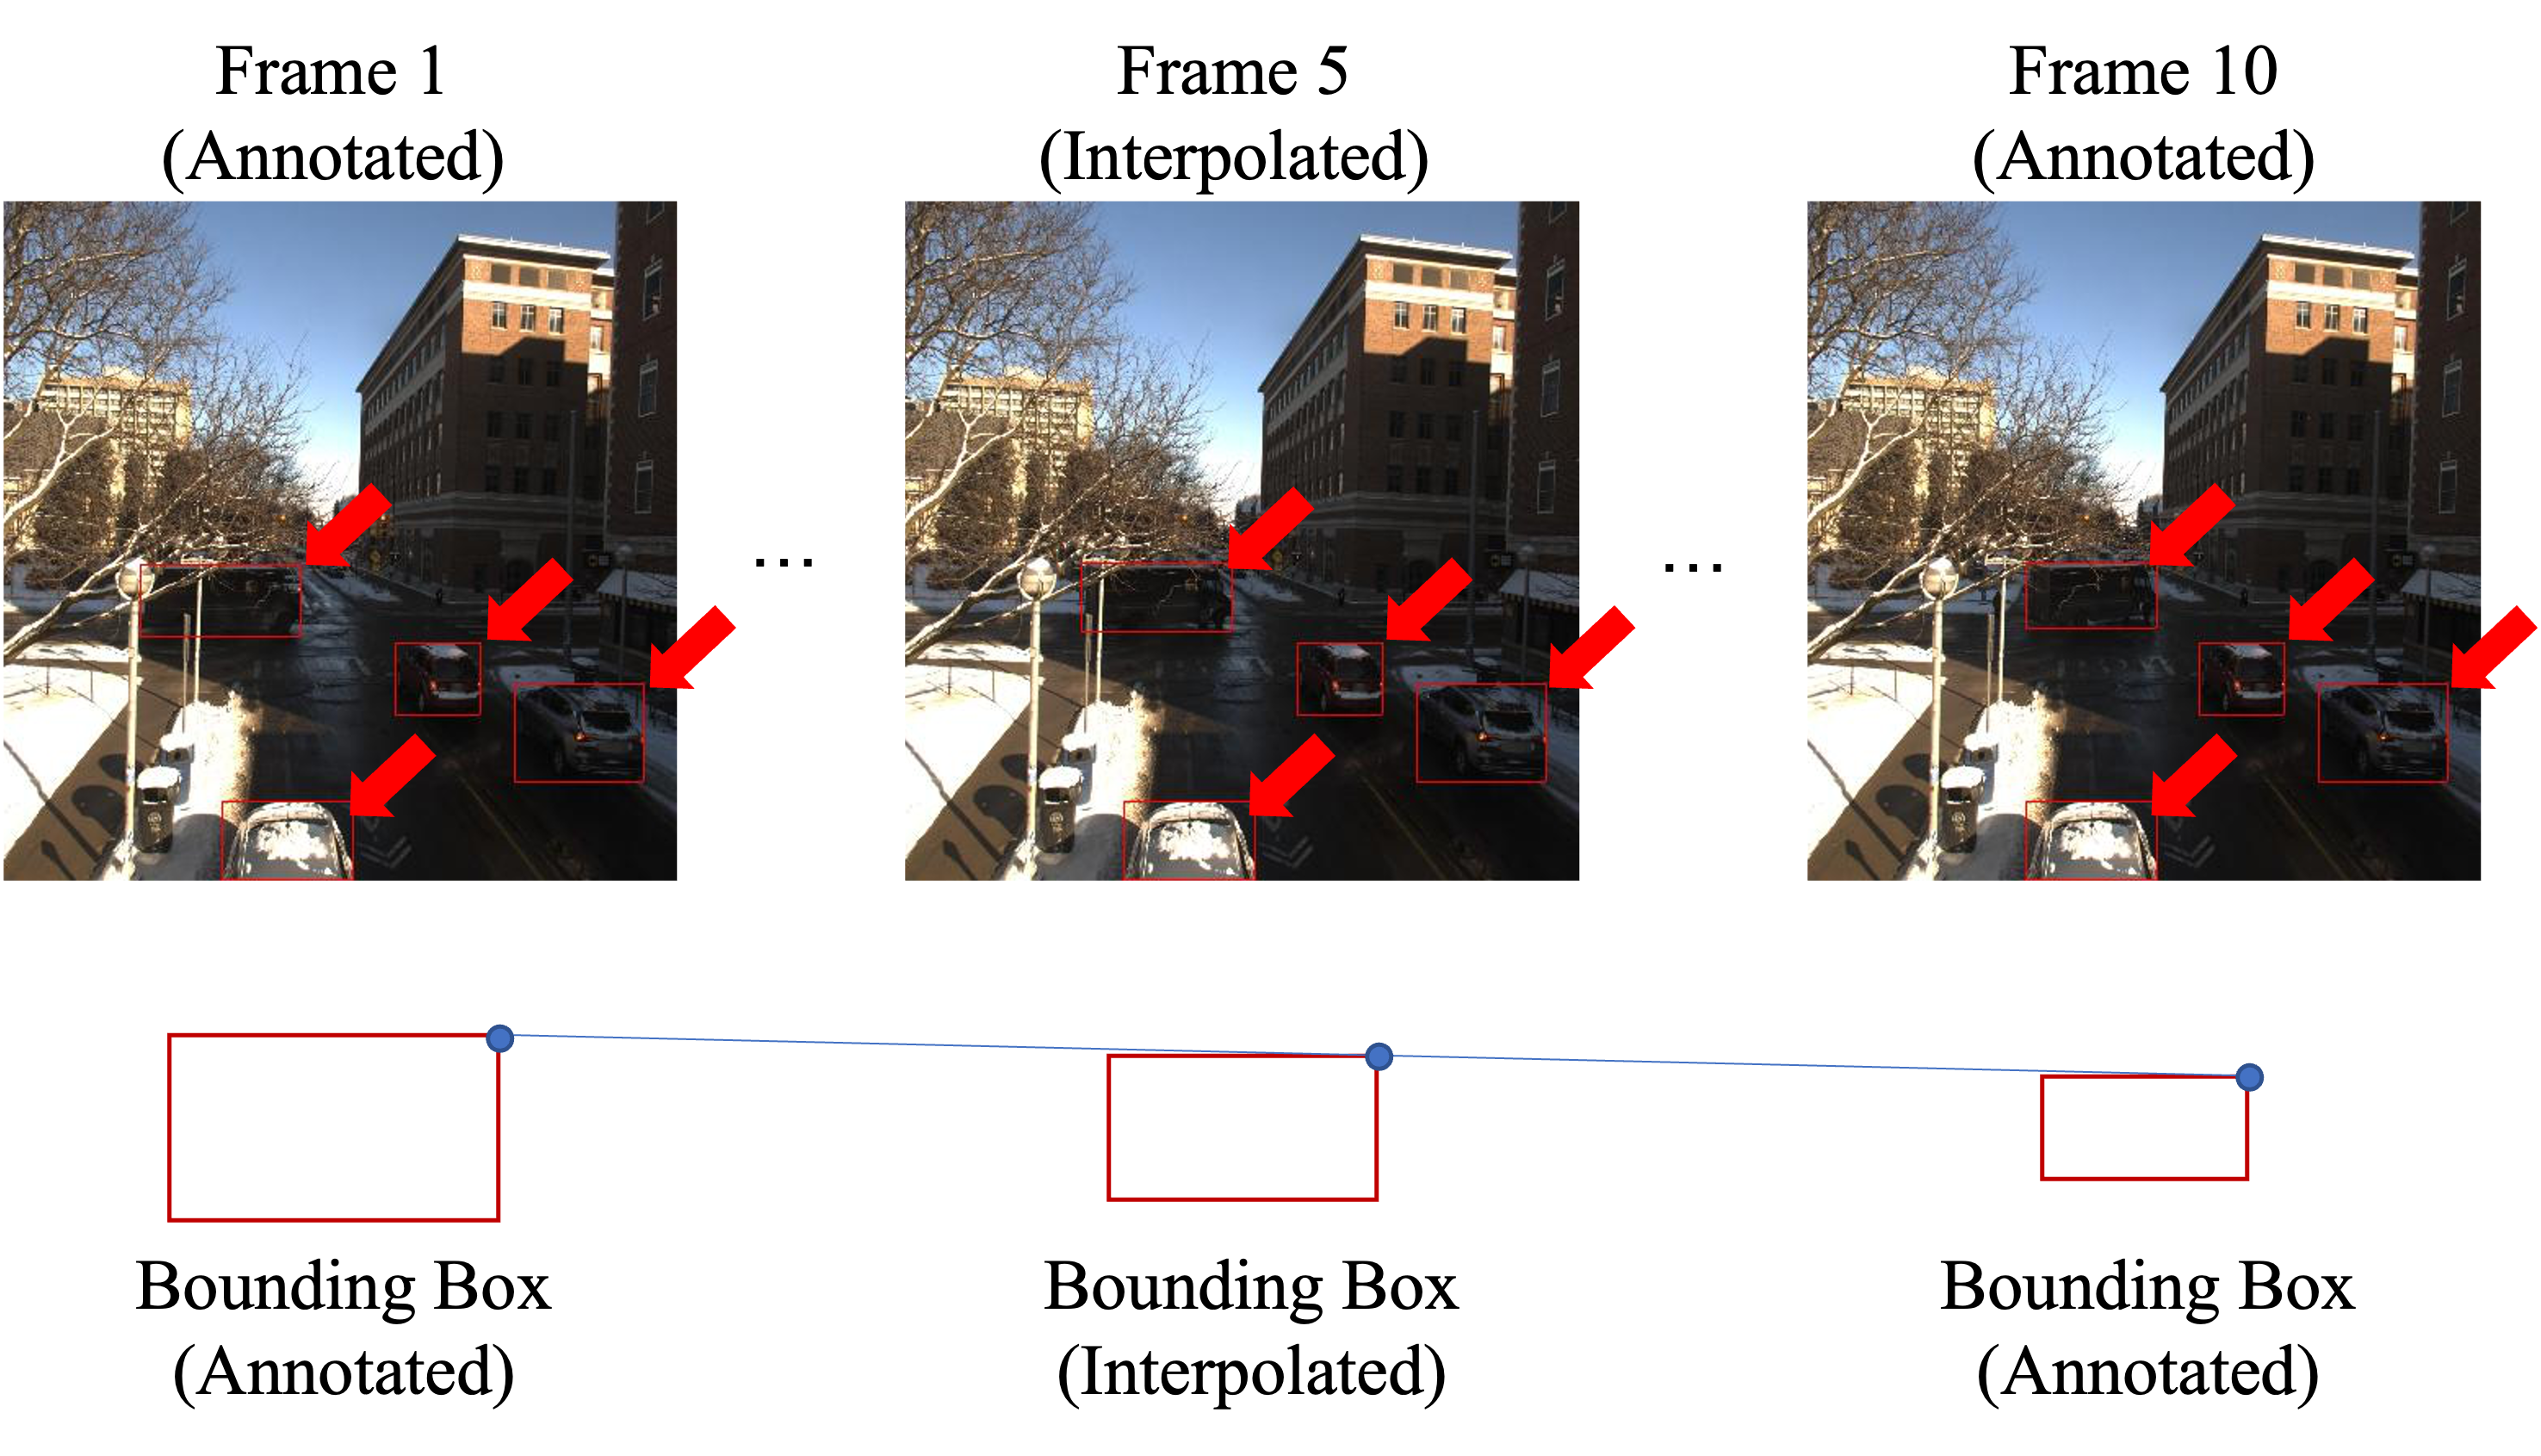}
	
	\caption{Label interpolation on a FOCAL sequence. Instead of annotating all objects in every frame, the annotator annotates Frame~1 and Frame~10 and interpolates the remaining labels. For interpolation, a simple linear mapping is used (bottom half).}
	
	\label{fig:interpolation-toy}
\end{figure}

We use the same experimental setup as in the main paper. In order to derive the cost of annotating single frames, we divide the total sequence cost by the effectively annotated frames assuming a fixed frame interpolation rate. For instance, a sequence of 100 sequentially correlated frames can be fully labeled by annotating every 10th frame in detail and interpolating the remaining frames with zero cost. Assuming the entire sequence took 10h to label, the cost-per-frame would be 1h (10h / 10 effective frames). We show the cost in hours for entropy sampling, margin sampling, and least confidence sampling with two, and five respectively (Figure~\ref{fig:cost-single-seq}). For a fair comparison, we additionally include our results with no interpolation that are discussed in the main paper. Complimentary to our previous observations, sequential approaches consistently outperform singular strategies regardless of the interpolation rate.
\begin{figure*}[t]
\centering
\includegraphics[scale=0.45]{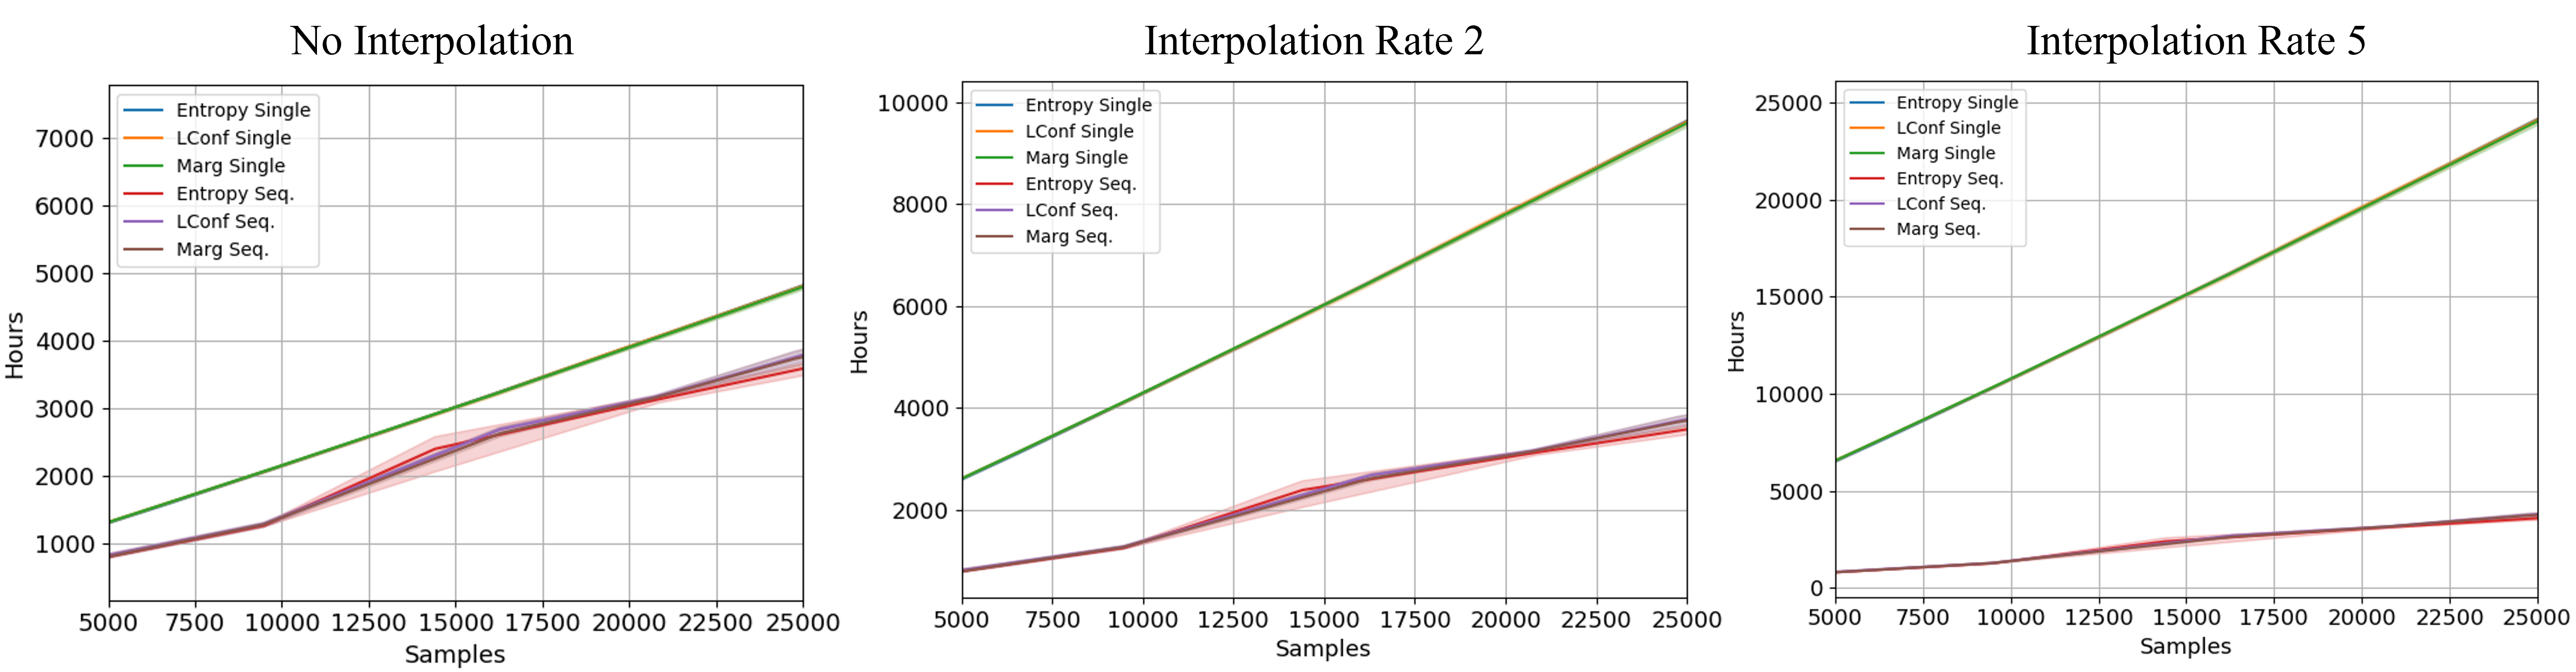}

\caption{Cost of sequential and single frame entropy sampling, margin sampling, and least confidence sampling on the FOCAL dataset when assuming different interpolation rates. Left: no interpolation. Middle: every second frame in sequence is annotated (rest interpolated). Right: every fifth frame in sequence is annotated (rest interpolated).}

\label{fig:cost-single-seq}
\end{figure*}
